# Supplementary material for: The Role of Energy Scales for the Structure of Ionic Liquids at Electrified Interfaces -- A Theory-Based Approach
Source: arXiv:2112.11511 ancillary file (2022-11-29)
Supplement: Supplementary file 1 [file supporting_info.pdf]

# Supporting information for: The Role of Energy Scales for the Structure of Ionic Liquids at Electrified Interfaces - A Theory-Based Approach.

Max Schammer,† Arnulf Latz,*,† and Birger Horstmann*,†

†*German Aerospace Center, Pfaffenwaldring 38-40, 70569 Stuttgart, Germany*

‡*Helmholtz Institute Ulm, Helmholtzstraße 11, 89081 Ulm, Germany*

¶*Universität Ulm, Albert-Einstein-Allee 47, 89081 Ulm, Germany*

E-mail: arnulf.latz@dlr.de; birger.horstmann@dlr.de

# Contents

**S-1 Transport Theory of Interacting Electrolytes** **S3**

S-1.1 Transport Theory: Functional Formalism . . . . . . . . . . . . . . . . . . . . . . S3

S-1.2 Constitutive Modelling for Interacting Liquid Electrolytes . . . . . . . . . . . . . . . S7

S-1.3 Gradient Expansion . . . . . . . . . . . . . . . . . . . . . . . . . . . . . . . . S8

S-1.4 Functional Derivative . . . . . . . . . . . . . . . . . . . . . . . . . . . . . . . . S10

**S-2 Non-Dimensional Formulation** **S11**

**S-3 Binary Ionic Liquid** **S14**

S-3.1 Interaction contribution to the chemical forces: Integral Form . . . . . . . . . . . . . S14

S-3.2 Special Case: Symmetric Ion species . . . . . . . . . . . . . . . . . . . . . . . . S16

S-3.3 Mean Steric Effect: Charge Saturation . . . . . . . . . . . . . . . . . . . . . . . . S16

S-3.3.1 Asymptotic Analysis for Small Potentials: EDL Charge and Differential Capacitance . . . . . . . . . . . . . . . . . . . . . . . . . . . . . . . S17

S-3.3.2 Asymptotic Analysis for Large Potentials: EDL Charge and Differential Capacitance . . . . . . . . . . . . . . . . . . . . . . . . . . . . . . . S18

S-3.3.3 Mean Volume Effect: Symmetric Ions . . . . . . . . . . . . . . . . . . . . S19

S-3.4 Non-Local Interactions: Charge Oscillations . . . . . . . . . . . . . . . . . . . . . S19

S-3.4.1 Perturbation Modes . . . . . . . . . . . . . . . . . . . . . . . . . . . . . S20

S-3.4.2 Analysis of the Phase Space of Screening Profiles . . . . . . . . . . . . . . S20

S-3.4.3 Limiting Cases . . . . . . . . . . . . . . . . . . . . . . . . . . . . . . . S24

S-3.4.4 Trivial Order Expansion . . . . . . . . . . . . . . . . . . . . . . . . . . . S25

S-3.4.5 Linear Order Expansion . . . . . . . . . . . . . . . . . . . . . . . . . . . S27

**S-4 Simulations** **S28**

S-4.1 Computational Details . . . . . . . . . . . . . . . . . . . . . . . . . . . . . . . S28

S-4.2 Binary Ionic Liquid PyrTFSI . . . . . . . . . . . . . . . . . . . . . . . . . . . . S29

**S-5 Relation to Experimental Methods** **S29**

**S-6 Simulation Results** **S30**

S-6.1 Phase Space of Screening Profiles . . . . . . . . . . . . . . . . . . . . . . . . . S30

S-6.2 Crystalline Limit: Ionic Phase-Separation . . . . . . . . . . . . . . . . . . . . . . . S31

S-6.3 Dependence of the Screening Profile on the Interface Potential . . . . . . . . . . . . S32

S-6.4 Meta Analysis of EDL-Descriptions . . . . . . . . . . . . . . . . . . . . . . . . . S33

**References** **S36**

# S-1 Transport Theory of Interacting Electrolytes

## S-1.1 Transport Theory: Functional Formalism

Recently, we derived a continuum theory which describes transport phenomena in highly concentrated electrolytes and ionic liquids (ILs).[S1] In this work, we extend the thermodynamically consistent framework from Ref. S1 by non-local interactions. Because derivation relies heavily on the methodology explained in great detail in Ref. S1, we reduce our derivation to the necessary logical steps, and refer to Ref. S1 for more details.

To account for non-local correlations, we generalize the local continuum description from Ref. S1 to a functional formalism. Hence, in this work, we discuss the evolution of field quantities having functional form, instead of the evolution of the corresponding local representations, *i.e.* volume-averaged field densities. For this purpose, we use global balancing laws to derive constitutive equations which take the form of functional derivatives and comprise non-local interactions.

We start our derivation of the generalized transport theory by formulating the global form of Cauchy's first equation ("force law"), which describes momentum evolution

$$\dot{\boldsymbol{G}} = \dot{\boldsymbol{G}}^{\text{int}} + \int \mathrm{dV}\ (\rho \boldsymbol{b} + \boldsymbol{\nabla}\sigma) = \int \mathrm{dV} \left( \frac{\delta \boldsymbol{G}^{\text{int}}}{\delta t} + \rho \boldsymbol{b} + \boldsymbol{\nabla}\sigma \right). \tag{S-1}$$

Here, $\boldsymbol{G}^{\text{int}}$ takes account for momentum contributions stemming from non-local interactions. These supplement the "bulk" momentum $\int \mathrm{dV}(\rho \boldsymbol{b} + \boldsymbol{\nabla}\boldsymbol{\sigma})$, determined by body-forces $\boldsymbol{b}$, and surface stresses comprised in the Cauchy stress tensor $\boldsymbol{\sigma}$. Next, we formulate the global form for energy balance,

$$\dot{\mathcal{E}} = \Pi + \mathcal{Q}. \tag{S-2}$$

Here, $\Pi(\boldsymbol{G})$ denotes the power of the forces acting on the system. Because this quantity is a function of the total momentum, it comprises contributions stemming from $\boldsymbol{G}^{\text{int}}$. As consequence, we split this quantity into $\Pi = \Pi^{\text{int}} + \int \mathrm{dV}\,[\rho \boldsymbol{b}\mathbf{v} + \boldsymbol{\nabla}(\boldsymbol{\sigma}^T\mathbf{v})]$. In contrast, the heating of the system maintains it's canonical form and is determined by a source-term and by fluxes of thermal and electromagnetic heating, $\mathcal{Q} = \int \mathrm{dV}\,\rho h - \boldsymbol{\nabla}(\boldsymbol{q} + \mathcal{E} \wedge \mathcal{H})$.

Apparently, the balance laws of momentum and energy (eqs. (S-1) and (S-2)) are mutually coupled. We exploit this coupling to derive balance of internal, non-kinematic energy, $\dot{\mathcal{U}} = \dot{\mathcal{E}} - \dot{\boldsymbol{G}}$. For this purpose, we make use of the relation $\boldsymbol{\nabla}(\boldsymbol{\sigma}^T\mathbf{v}) = \mathbf{v}(\boldsymbol{\nabla}\boldsymbol{\sigma}^T) + \boldsymbol{\sigma} : \operatorname{grad}\mathbf{v}$, and solve the momentum equation (eq. (S-1)) for $\int \mathrm{dV}\,\rho\mathbf{bv} = \int \mathrm{dV}\,\mathbf{v}(\delta\boldsymbol{G}/\delta t - \delta\boldsymbol{G}^{\text{int}}/\delta t - \boldsymbol{\nabla}\boldsymbol{\sigma})$, such that

$$\dot{\mathcal{U}} = \Pi^{\text{int}} + \int \mathrm{dV}[-\delta\boldsymbol{G}^{\text{int}}/\delta t \cdot \mathbf{v} + \boldsymbol{\sigma} : \operatorname{grad}\mathbf{v} - \boldsymbol{\nabla}(\boldsymbol{q} + \mathcal{E} \wedge \mathcal{H}) + \rho h] \tag{S-3}$$

Our next step is to ensure that our description complies with the second axiom of thermodynamics. For this purpose, we split the entropy of the system into a bulk-term and a functional term, *viz.* $\mathcal{S} = \mathcal{S}^{\text{int}} + \int \mathrm{dV}\,\rho s$. Here, we assume constant temperature $T$ of the system. Hence, the irreversible loss of energy is $T \cdot \mathcal{S} = T \cdot \mathcal{S}^{\text{int}} + \int \mathrm{dV}\,\rho s T$. We express the second axiom of thermodynamics via

$$\dot{\mathcal{S}} = \dot{\mathcal{S}}^{\text{int}} + \int \mathrm{dV}\,\rho\dot{s} \geq \int \mathrm{dV}\left(-\boldsymbol{\nabla}\boldsymbol{\xi}_s + \frac{\rho h}{T}\right). \tag{S-4}$$

Apparently, entropy changes due to entropic fluxes $\boldsymbol{\xi}_s$, and due to heating-process $\rho h/T$ (entropic source-term). The right side of eq. (S-4) measures the deviation from equilibrium. This suggests

that we define the residual quantity as measure for the rate of irreversible entropy production,

$$\int \mathrm{dV}\, \mathcal{R} = T\dot{\mathcal{S}} + \int \mathrm{dV}\, \left(T\boldsymbol{\nabla}\boldsymbol{\xi}_s - \rho h\right) \tag{S-5}$$

$$= T\dot{\mathcal{S}} - \dot{\mathcal{U}} + \Pi^{\mathrm{int}} + \int \mathrm{dV}\, \left(T\boldsymbol{\nabla}\boldsymbol{\xi}_s - \mathbf{v}\frac{\delta \boldsymbol{G}^{\mathrm{int}}}{\delta t} + \boldsymbol{\sigma} : \mathrm{grad}\mathbf{v} - \boldsymbol{\nabla}\boldsymbol{q} + \boldsymbol{\nabla}\left(\mathcal{H} \wedge \mathcal{E}\right)\right). \tag{S-6}$$

Here, we used eq. (S-3) to substitute for the quantity $\int \mathrm{dV}\, \rho h$. Furthermore, we make the identification $\Pi^{\mathrm{int}} = \int \mathrm{dV}\, \mathbf{v} \cdot \delta\boldsymbol{G}^{\mathrm{int}}/\delta t$, as appearing on the right side of eq. (S-6). However, focal quantity in our framework is the Helmholtz free energy $F = \mathcal{U} - T\mathcal{S}$, *i.e.* the Legendre transformed quantity with respect to internal energy. Therefore, we reformulate eq. (S-6) such that

$$\int \mathrm{dV}\, \mathcal{R} = -\dot{F} - \dot{T}\mathcal{S} + \int \mathrm{dV}\, \left(T\boldsymbol{\nabla}\boldsymbol{\xi}_s + \boldsymbol{\sigma} : \mathrm{grad}\mathbf{v} - \boldsymbol{\nabla}\boldsymbol{q} + \boldsymbol{\nabla}\left(\mathcal{H} \wedge \mathcal{E}\right)\right). \tag{S-7}$$

Equation (S-7) determines the constitutive equations subject to the form of $\dot{F}(\Upsilon)$, *i.e.* subject to the set of material variables $\Upsilon$ which characterize the system. In order to account for molecular interactions, we expand the free energy of the system via eq. (1),

$$F = F^{\mathrm{int}} + \int \mathrm{dV}\, \rho\varphi_{\mathrm{H}}. \tag{S-8}$$

We use a canonical hydrodynamic description for polarizable liquids, $\Upsilon = \{\boldsymbol{D}, \boldsymbol{B}, T, c_\alpha, \boldsymbol{\kappa}\}$,[S1,S2] such that the variation of the free energy becomes

$$\delta F = \int \mathrm{dV}\, \mathcal{E} \cdot \delta\boldsymbol{D} + \mathcal{H} \cdot \delta\boldsymbol{B} + \rho s \cdot \delta T + \sum_{\alpha=1}^{\mathrm{N}} \mu_\alpha \cdot \delta c_\alpha + \rho\varphi_{\mathrm{H}} \cdot \boldsymbol{\nabla}\mathbf{v}, \tag{S-9}$$

Here, $\boldsymbol{\kappa}$ denotes the strain-rate tensor which constitutes systems in liquid state.

Next, we derive the constitutive equations following from our functional approach. For this purpose, we first evaluate $\dot{F}$ in eq. (S-7) with respect to the material law $\Upsilon$. Next, we use mass balance $\dot{c}_\alpha = -\boldsymbol{\nabla}\mathcal{N}_\alpha - c_\alpha\boldsymbol{\nabla}\mathbf{v}$, and substitute the entropic flux-term via $T\boldsymbol{\nabla}\boldsymbol{\xi}_s = -\boldsymbol{\xi}_s\boldsymbol{\nabla}T + \boldsymbol{\nabla}\boldsymbol{q} - \boldsymbol{\nabla}\sum_{\alpha=1}^{\mathrm{N}} \mu_\alpha \mathcal{N}_\alpha$.[S1] Finally, we re-express the electromagnetic Poynting flux by $\boldsymbol{\nabla}\left(\mathcal{H} \wedge \mathcal{E}\right) = \mathcal{E}\mathcal{J} + \mathcal{E}\dot{\boldsymbol{D}} + \mathcal{H}\dot{\boldsymbol{B}} +$

$[(\mathcal{E}\boldsymbol{D} + \mathcal{H}\boldsymbol{B})\,\mathbf{Id} - \mathcal{E} \otimes \boldsymbol{D} - \mathcal{H} \otimes \boldsymbol{B}] : \mathrm{grad}\mathbf{v}$.[S1,S3] Altogether, we find for the constitutive equations,

$$\rho s = -\rho\frac{\partial \varphi_{\mathrm{H}}}{\partial T} - \frac{\delta F^{\mathrm{int}}}{\delta T}, \tag{S-10}$$

$$\mathcal{E} = \rho\frac{\partial \varphi_{\mathrm{H}}}{\partial \boldsymbol{D}} + \frac{\delta F^{\mathrm{int}}}{\delta \boldsymbol{D}}, \tag{S-11}$$

$$\mathcal{H} = \rho\frac{\partial \varphi_{\mathrm{H}}}{\partial \boldsymbol{B}} + \frac{\delta F^{\mathrm{int}}}{\delta \boldsymbol{B}}, \tag{S-12}$$

$$\mu_\alpha = \frac{\partial(\rho\varphi_{\mathrm{H}})}{\partial c_\alpha} + \frac{\delta F^{\mathrm{int}}}{\delta c_\alpha}. \tag{S-13}$$

Equations (S-10) to (S-13) are substituted by $\partial\varphi_{\mathrm{H}}/\partial\boldsymbol{\kappa} = \delta F^{\mathrm{int}}/\delta\boldsymbol{\kappa} = 0$, and by the constitutive equation for the stress tensor,

$$\boldsymbol{\sigma} = \boldsymbol{\tau} - \left(\sum_{\alpha=1}^{\mathrm{N}} c_\alpha \left[\frac{\partial(\rho\varphi_{\mathrm{H}})}{\partial c_\alpha} + \frac{\delta F^{\mathrm{int}}}{\delta c_\alpha}\right] - \rho\varphi_{\mathrm{H}} + \mathcal{E}\boldsymbol{D} + \mathcal{H}\boldsymbol{B}\right) \cdot \mathbf{Id} + \mathcal{E} \otimes \boldsymbol{D} + \mathcal{H} \otimes \boldsymbol{B}. \tag{S-14}$$

Here $\boldsymbol{\tau}(\boldsymbol{\kappa}) = \lambda\boldsymbol{\nabla}\mathbf{v} \cdot \mathbf{Id} + 2\eta \cdot \boldsymbol{\kappa}_{\mathrm{tf}}$ describes the viscosity tensor, where $\boldsymbol{\kappa} = [\mathrm{grad}\,\mathbf{v} + (\mathrm{grad}\,\mathbf{v})^{\mathrm{T}}]/2 = \boldsymbol{\nabla}\mathbf{v} \cdot \mathbf{Id}/3 + \boldsymbol{\kappa}_{\mathrm{tf}}$ is the strain-rate tensor and $\mathbf{v}$ is the center-of-mass convection velocity.[S1]

Since we neglect magnetic fields,[S4] the residual expression for the entropy production rate (after evaluation of the constitutive equations) becomes $\int \mathrm{dV}\mathcal{R} = \int \mathrm{dV}\,[-\boldsymbol{\mathcal{J}}\boldsymbol{\nabla}\Phi - \sum_{\alpha=1}^{\mathrm{N}} \mathcal{N}_\alpha\boldsymbol{\nabla}\mu_\alpha - \boldsymbol{\xi}_s\boldsymbol{\nabla}T + \boldsymbol{\tau} : \boldsymbol{\kappa}]$. Here, $\boldsymbol{\tau}(\boldsymbol{\kappa}) = \lambda\boldsymbol{\nabla}\mathbf{v} \cdot \mathbf{Id} + 2\eta \cdot \boldsymbol{\kappa}_{\mathrm{tf}}$ denotes the viscosity tensor, which determines the constitutive equation for the stress-tensor (where $\boldsymbol{\kappa}_{\mathrm{tf}}$ is the trace-free part of the strain-rate tensor), $\boldsymbol{\sigma} = \boldsymbol{\tau} - (\sum_{\alpha=1}^{\mathrm{N}} \mu_\alpha c_\alpha - \rho\varphi_{\mathrm{H}} + \boldsymbol{E}\boldsymbol{D}) \cdot \mathbf{Id} + \boldsymbol{E} \otimes \boldsymbol{D}$. The evaluation of the constitutive equation for the chemical potential as described in the main text (see section II A and Ref. S1) yields for the electrochemical forces (defined by $\boldsymbol{\nabla}\mu_\alpha^{\mathrm{el}} = \boldsymbol{\nabla}(\mu_\alpha + Fz_\alpha\boldsymbol{\nabla}\Phi)$), the following result

$$\boldsymbol{\nabla}\mu_\alpha^{\mathrm{el}} = \sum_{\beta=1}^{\mathrm{N}} \left(\delta_\alpha^\beta - \nu_\alpha c_\beta\right) \cdot \boldsymbol{\nabla}\left(Fz_\beta\Phi + \frac{\delta F^{\mathrm{int}}}{\delta c_\beta}\right) - \nu_\alpha\left(\sum_{\beta=1}^{\mathrm{N}} \frac{\delta F^{\mathrm{int}}}{\delta c_\beta}\boldsymbol{\nabla}c_\beta - \frac{\delta \boldsymbol{G}^{\mathrm{int}}}{\delta t}\right) + $$
$$+ RT\left(\boldsymbol{\nabla}\ln c_\alpha\nu_\alpha - \nu_\alpha\boldsymbol{\nabla}c\right). \tag{S-15}$$

As consequence, the Gibbs-Duhem equation becomes $\sum_{\alpha=1}^{\mathrm{N}} c_\alpha\boldsymbol{\nabla}\mu_\alpha^{\mathrm{el}} = \boldsymbol{\nabla}\boldsymbol{\tau} - \nu_\alpha(\sum_{\beta=1}^{\mathrm{N}} \delta F^{\mathrm{int}}/\delta c_\beta \cdot \boldsymbol{\nabla}c_\beta - \delta\boldsymbol{G}^{\mathrm{int}}/\delta t)$. However, because we assume that this relation is trivial in the stationary state, we

conclude

$$\dot{\boldsymbol{G}}^{\text{int}} = \int \mathrm{dV} \sum_{\alpha=1}^{\mathrm{N}} \frac{\delta F^{\text{int}}}{\delta c_\alpha} \cdot \boldsymbol{\nabla} c_\alpha. \tag{S-16}$$

## S-1.2 Constitutive Modelling for Interacting Liquid Electrolytes

We state the Helmholtz free energy for liquid electrolytes supplemented by a universal non-local interaction,

$$F = F^{\text{int}} + \int \mathrm{dV}\, \rho\varphi_{\mathrm{H}} = F^{\text{int}} + \int \mathrm{dV} \frac{\boldsymbol{ED}}{2} + \frac{\mathcal{K}}{2}\left(1 - \sum_{\alpha=1}^{\mathrm{N}} \nu_\alpha^0 c_\alpha\right)^2 + RT \sum_{\alpha=1}^{\mathrm{N}} c_\alpha \ln(c_\alpha \nu_\alpha), \tag{S-17}$$

where the electric field is $\boldsymbol{E} = \boldsymbol{D}/\varepsilon_0\varepsilon_{\mathrm{R}}$. The second term comprises volumetric energy contributions. We express this term by expansion around a stable reference configuration parametrized by $\nu_\alpha^0$ and $\mathcal{K}$ constitutes a Lagrange multiplier. To take account for asymmetric volumes of the ions, we express the entropy of mixture using volume fractions $c_\alpha \nu_\alpha$, instead of mole fractions $c_\alpha/c$.[S5] This "Flory-Huggins"-approach is based on a modified statistics,[S6] which favours equal volumes for each species instead of equal number of molecules, and accounts for the averaged impact of strong short range repulsion on particle distributions. Within the framework Ref. S1 this change is captured by the bulk activity coefficients $f_\alpha$ given by the partial molar volumes $f_\alpha = \nu_\alpha$. In Ref. S1 we show that the chemical potentials

$$\mu_\alpha = RT\,(1 + \ln c_\alpha \nu_\alpha) + \frac{\delta F^{\text{int}}}{\delta c_\alpha} - \mathcal{K}\nu_\alpha^0 \left(1 - \sum_{\beta=1}^{\mathrm{N}} c_\beta \nu_\beta^0\right), \tag{S-18}$$

depend on elastic properties through the last term. As discussed in our previous work[S1] and in Ref. S7 for hardly compressible electrolytes, this elastic energy represents a linear pressure contribution and the Lagrange multiplier $\mathcal{K}$ is found to be the Bulk modulus. In this work, we assume the incompressible limit $\mathcal{K}\to\infty$. This implies that the thermodynamic partial molar volumes $\nu_\alpha$

become pressure independent and approach the partial molar volumes in the reference state,

$$\lim_{\mathcal{K}\to\infty} \nu_\alpha = \nu_\alpha^0. \tag{S-19}$$

We take account for local conservation of volume via the Euler equation for the volume,

$$\sum_{\alpha=1}^{N} c_\alpha \nu_\alpha = 1. \tag{S-20}$$

The elastic term in the chemical potentials (see eq. (S-18)) is constrained by the assumption of mechanical equilibrium div $\boldsymbol{\sigma} = 0$. Then, eq. (S-14) implies $\mathcal{K} \sum_{\beta=1}^{N} \nu_\beta \cdot \boldsymbol{\nabla} c_\beta = -\varrho \boldsymbol{\nabla} \Phi - RT \cdot \boldsymbol{\nabla} c - \boldsymbol{\nabla} \sum_{\beta=1}^{N} c_\beta \cdot \delta F^{\text{int}} / \delta c_\beta$ and the electrochemical forces $\boldsymbol{\nabla} \mu_\alpha^{\text{el}} = \boldsymbol{\nabla} \mu_\alpha + F z_\alpha \boldsymbol{\nabla} \Phi$ become

$$\boldsymbol{\nabla} \mu_\alpha^{\text{el}} = \nu_\alpha \boldsymbol{\nabla} \boldsymbol{\tau} + \sum_{\beta=1}^{N} \left( \delta_\alpha^\beta - \nu_\alpha c_\beta \right) \boldsymbol{\nabla} \left( F z_\beta \Phi + \frac{\delta F^{\text{int}}}{\delta c_\beta} \right) + RT \left( \boldsymbol{\nabla} \ln \left[ c_\alpha \nu_\alpha \right] - \nu_\alpha \boldsymbol{\nabla} c \right), \tag{S-21}$$

where $\boldsymbol{\nabla}\boldsymbol{\tau} = (\lambda + \eta/3) \boldsymbol{\nabla}(\boldsymbol{\nabla} \mathbf{v}) + \eta \cdot \boldsymbol{\nabla}^2 \mathbf{v}$. Thus, in this limit, we obtain inter-species couplings, in agreement with the Gibbs-Duhem relation,

$$\sum_{\alpha=1}^{N} c_\alpha \cdot \boldsymbol{\nabla} \mu_\alpha^{\text{el}} = \boldsymbol{\nabla} \boldsymbol{\tau}. \tag{S-22}$$

### S-1.3 Gradient Expansion

In this section, we derive the gradient expansion of the interaction functional $F^{\text{int}}$, as stated in the main text, see eq. (5). This approximation reproduces results which were recently proposed by mean field theories (MFTs).[S8] Furthermore, the resulting transport equations are susceptible to analytical techniques.

For completeness, we restate the interaction functional $F^{\text{int}}[c_\alpha]$ which is determined by the

hardcore potential $\mathcal{F}_{\alpha\beta}$,

$$F^{\text{int}} = \frac{1}{2}\sum_{\alpha,\beta}^{\text{N}} \int_{\Omega_y} \mathrm{d}y\; c_\alpha(y) \left( \int_{\Omega_x} \mathrm{d}x\; \mathcal{F}_{\alpha\beta}(|x-y|) c_\beta(x) \right). \tag{S-23}$$

The crucial assumption in our derivation is that the interaction potential $\mathcal{F}_{\alpha\beta}$ is of short-range, *i.e.* the correlations decay after some ion-sizes. We evaluate this assumption observing that the variable "$y$", which appears in the bracked term on the right side of eq. (S-23), is merely a constant. Thus, for any position "$y$", we reduce the integration limits of the bracked convolution to the interval $\Omega_x = [y - \sigma_{\alpha\beta}; y + \sigma_{\alpha\beta}]$, where $0 < \sigma_{\alpha\beta} \ll |y|$,

$$F^{\text{int}}[c_\gamma] = \frac{1}{2}\sum_{\alpha,\beta} \int_{\Omega_y} \mathrm{d}y\; c_\alpha(y) \left( \int_{y-\sigma_{\alpha\beta}}^{y+\sigma_{\alpha\beta}} \mathrm{d}x\; \mathcal{F}_{\alpha\beta}\,(|x-y|)\; c_\beta(x) \right). \tag{S-24}$$

Next, we make a coordinate transformation of the bracked integral using relative coordinates defined by $\varepsilon = x - y$, where $x = g(\varepsilon) = \varepsilon + y$ and $\varepsilon = g^{-1}(x_0) = x_0 - y$. Note that the integration limits transform according to ($g^{-1}(y - \sigma_{\alpha\beta}) = -\sigma_{\alpha\beta}$ and $g^{-1}(y + \sigma_{\alpha\beta}) = \sigma_{\alpha\beta}$). Hence, we find

$$F^{\text{int}}[c_\gamma] = \frac{1}{2}\sum_{\alpha,\beta} \int_{\Omega_y} \mathrm{d}y\; c_\alpha(y) \left( \int_{-\sigma_{\alpha\beta}}^{\sigma_{\alpha\beta}} \mathrm{d}\varepsilon\; \mathcal{F}_{\alpha\beta}\,(|\varepsilon|)\; c_\beta(y+\varepsilon) \right). \tag{S-25}$$

Our basic assumption implies that $\varepsilon \ll y$. We make use of this property and Taylor-expand the ion-concentration according to $c_\beta(y+\varepsilon) = \sum_{n=0}^{\infty} \varepsilon^n/n! \cdot \nabla^n c_\beta(y)$, such that eq. (S-25) decouples into the product of two independent integrals

$$F^{\text{int}}[c_\gamma] = \frac{1}{2}\sum_{\alpha,\beta}\sum_{n=0}^{\infty} \frac{1}{n!} \left( \int_{-\sigma_{\alpha\beta}}^{\sigma_{\alpha\beta}} \mathrm{d}\varepsilon\; \mathcal{F}_{\alpha\beta}\,(|\varepsilon|)\; \varepsilon^n \right) \cdot \left( \int_{\Omega_y} \mathrm{d}y\; c_\alpha(y) \cdot \nabla^n c_\beta(y) \right). \tag{S-26}$$

The left integral, which comprises the molecular interactions, exhibits spherical symmetry. This symmetry implies that all integrals with odd modes $n$ vanish identically. Therefore, the

integration limits in all remaining terms can be translated according to, $\int_{-\sigma_{\alpha\beta}}^{\sigma_{\alpha\beta}} \mathrm{d}\varepsilon\, \mathcal{F}_{\alpha\beta}\,(|\varepsilon|)\, \varepsilon^{2n} = \int_{0}^{\sigma_{\alpha\beta}} \mathrm{d}\varepsilon\, \mathcal{F}_{\alpha\beta}\,(|\varepsilon|)\, \varepsilon^{2n}$. Hence,

$$F^{\mathrm{int}}[c_\gamma] = \frac{1}{2} \sum_{\alpha,\beta} \sum_{n=0}^{\infty} \Gamma_{\alpha\beta}^{2n} \cdot \int_{\Omega_y} \mathrm{d}y\, c_\alpha(y) \cdot \boldsymbol{\nabla}^{2n} c_\beta(y), \tag{S-27}$$

where

$$\Gamma_{\alpha\beta}^{n} = \frac{1}{(n!)} \int_{0}^{\sigma_{\alpha\beta}} \mathrm{d}\varepsilon\, \mathcal{F}_{\alpha\beta}(|\varepsilon|) \cdot \varepsilon^{n}. \tag{S-28}$$

Finally, we note that this expansion can be written in an alternative way. For this purpose, we observe that the unbalanced action of the Nabla-operator on one concentration in eq. (S-27) can be symmetrized if all derivatives $\boldsymbol{\nabla}^n c_\gamma|_\Omega = 0$ vanish at the boundaries of the integration-domain. In this case, the $n$-fold application of the method of integration by parts yields

$$F^{\mathrm{int}}[c_\gamma] = \frac{1}{2} \sum_{\alpha,\beta} \sum_{n=0}^{\infty} (-1)^n \cdot \Gamma_{\alpha\beta}^{2n} \cdot \int_{\Omega_y} \mathrm{d}y\, \left(\boldsymbol{\nabla}^n c_\alpha\right) \cdot \left(\boldsymbol{\nabla}^n c_\beta\right). \tag{S-29}$$

If the derivatives do not vanish at the boundary, then corrections to the above terms in the form of surface-integrals emerge.

### S-1.4 Functional Derivative

Many quantities arising in a functional formalism follow from calculus of variations, *i.e.* functional derivatives. For example, the chemical potentials appearing in our extended framework are defined via the constitutive equation $\mu_\alpha = \delta F^{\mathrm{int}}/\delta c_\alpha$, see eq. (S-13). Here, we give briefly sketch how the functional derivative can be defined and derive the functional derivative for the chemical potentials with respect to the free energy above, see eqs. (S-27) and (S-28).

Usually,[S9] the functional derivative of a quantity $F^{\mathrm{int}} = \int_{\Omega_x} \mathrm{d}x\, \Psi(c_\gamma, \boldsymbol{\nabla}^n c_\gamma)$ is defined via an

arbitrary, auxiliary function $\phi(x)$, such that

$$\int_{\Omega_x} \mathrm{d}x \, \frac{\delta F^{\mathrm{int}}}{\delta c_\gamma} \cdot \phi = \frac{\mathrm{d}}{\mathrm{d}\varepsilon}\bigg|_{\varepsilon=0} \left( \int_{\Omega_x} \mathrm{d}x \, \Psi\left(c_\gamma + \varepsilon\phi, \boldsymbol{\nabla}^n c_\gamma + \varepsilon \boldsymbol{\nabla}^n \phi\right) \right) =$$

$$= \int_{\Omega_x} \mathrm{d}x \left( \frac{\partial \Psi}{\partial c_\gamma} + \sum_{i=1}^{\infty} (-1)^i \cdot \boldsymbol{\nabla}^i \left[ \frac{\partial \Psi}{\partial \left(\boldsymbol{\nabla}^i c_\gamma\right)} \right] \right) \cdot \phi. \quad \text{(S-30)}$$

Hence, considering the functional $F^{\mathrm{int}} = 1/2 \cdot \sum_{\alpha,\beta} \sum_{n=0}^{\infty} \Gamma_{\alpha\beta}^{2n} \cdot c_\alpha \cdot \boldsymbol{\nabla}^{2n} c_\beta$, we find for the individual terms on the right hand side of eq. (S-30),

$$\frac{\partial \Psi}{\partial c_\gamma} = \sum_\alpha \Gamma_{\gamma\alpha}^0 \cdot c_\alpha + \frac{1}{2} \sum_\alpha \sum_{n=1}^{\infty} \Gamma_{\gamma\alpha}^n \cdot \boldsymbol{\nabla}^{2n} c_\alpha, \quad \text{(S-31)}$$

and

$$\sum_{i=1}^{\infty} (-1)^i \cdot \boldsymbol{\nabla}^i \frac{\partial \Psi}{\partial(\boldsymbol{\nabla}^i c_\gamma)} = \frac{1}{2} \sum_{i=1}^{\infty} (-1)^i \cdot \boldsymbol{\nabla}^i \left( \sum_{\alpha,\beta} \sum_{n=1}^{\infty} \Gamma_{\alpha\beta}^n \cdot c_\alpha \cdot \delta_\gamma^\beta \cdot \delta_i^{2n} \right) = \frac{1}{2} \sum_\alpha \sum_{n=1}^{\infty} \Gamma_{\gamma\alpha}^{2n} \cdot \boldsymbol{\nabla}^{2n} c_\alpha. \quad \text{(S-32)}$$

Therefore, by insertion of eqs. (S-31) and (S-32) into eq. (S-30) we find,

$$\frac{\delta F^{\mathrm{int}}}{\delta c_\alpha(z)} = \sum_{\beta=1}^{\mathrm{N}} \sum_{n=0}^{\infty} \Gamma_{\alpha\beta}^{2n} \cdot \boldsymbol{\nabla}^{2n} c_\beta(z). \quad \text{(S-33)}$$

Hence, with the Ansatz eq. (9) for the interaction functional $F^{\mathrm{int}}$, the complete free energy for IL electrolytes becomes

$$F = \int \mathrm{d}V \left[ \frac{\boldsymbol{ED}}{2} + RT \sum_{\alpha=1}^{\mathrm{N}} c_\alpha \ln(c_\alpha \nu_\alpha) + \; + \frac{\mathcal{K}}{2} \left( 1 - \sum_{\alpha=1}^{\mathrm{N}} c_\alpha \nu_\alpha^0 \right)^2 + \frac{1}{2} \sum_{\alpha,\beta}^{\mathrm{N}} \sum_{n=0}^{\infty} \Gamma_{\alpha\beta}^{2n} c_\alpha \cdot \boldsymbol{\nabla}^{2n} c_\beta \right]. \quad \text{(S-34)}$$

## S-2 Non-Dimensional Formulation

In this section we present our choice for the non-dimensionalization of quantities discussed in section II D. In particular, we show that our definitions account for different ion-sizes of the species

and reproduce the standard expressions used in the literature.

The choice of non-dimensionalized quantities influences the appearance of the corresponding transport equations. As consequence, this also influences the definition of subsequent parameters emerging from the framework (e.g., the Debye-length $L_\mathrm{D}$ or the energy scales $E_\mathrm{th}$ and $E_\mathrm{el}$). However, in order to properly reproduce "canonical" expressions for these quantities appearing in the literature, we choose our dimensional gauging appropriately.

Here, we use a standard gauge for the electrolyte electric potential,[S5] $\tilde{\Phi} = Fz_+\Phi/RT = e\Phi/k_\mathrm{B}T$. In the main text, we showed that the Debye-length $L_\mathrm{D}$ emerges naturally as a generic length gauge within our framework, , by substitution of the charge density $\tilde{\varrho}$ and of the electric potential $\tilde{\Phi}$ into the Poisson equation $\varrho = -\boldsymbol{\nabla}\varepsilon_\mathrm{R}\varepsilon_0\boldsymbol{\nabla}\Phi$, see eq. (17). Note that in the case of symmetric ion-species, $\gamma_\pm = 1/2$, the Debye-length becomes $L_\mathrm{D} = \sqrt{k_\mathrm{B}T\varepsilon_0\varepsilon_\mathrm{R}/2N_\mathrm{A}c^\mathrm{b}(ez_+)^2}$, which reproduces the canonical textbook-expression from the literature (see, e.g., Ref. S10).

With this length scale, we non-dimensionalize our grid, *viz.* $\tilde{x} = x/L_\mathrm{D}$ and $\tilde{\boldsymbol{\nabla}} = L_\mathrm{D}\cdot\boldsymbol{\nabla}$, and obtain the dimensionless Poisson-equation, $\tilde{\varrho} = -\tilde{\boldsymbol{\nabla}}^2\tilde{\Phi}$.

Our theory also contains a generalized Bjerrum-length $L_\mathrm{B}$, which measures the distance at which the electrostatic energy and the thermal energy become comparable,

$$L_\mathrm{B} = \frac{(ez_+)^2}{k_B T\varepsilon_0\varepsilon_\mathrm{R}\tilde{c}^\mathrm{b}} = \frac{a^3}{L_\mathrm{D}^2}. \tag{S-35}$$

Next, we substitute $\tilde{\Phi}$ into eq. (15), and assume the limiting case far away from the electrode. Hence, we approximate the logarithmic term in around the equilibrium state such that $\gamma_+\ln(c_-/c^\mathrm{b}) - \gamma_-\ln(c_+/c^\mathrm{b}) \approx -\varrho\nu\cdot[(\gamma_+)^2+(\gamma_-)^2]/Fz_+$. Altogether, eq. (15) becomes

$$\boldsymbol{\nabla}\tilde{\mu}_\mathrm{IL} = \boldsymbol{\nabla}\left[\tilde{\Phi} - \frac{1}{RT}\left(\nu_+\frac{\delta F^\mathrm{int}}{\delta c_-} - \nu_-\frac{\delta F^\mathrm{int}}{\delta c_+}\right) + \frac{\varrho\nu[(\gamma_+)^2+(\gamma_-)^2]}{Fz_+}\right], \tag{S-36}$$

where we used the non-dimensionalization $\tilde{\mu}_\alpha = \mu_\alpha/RT$. Note that $\delta F^\mathrm{int}/\delta c_+\cdot 1/RT$ is non-dimensional. The right side suggests defining $\tilde{\varrho} = \varrho\nu[(\gamma_+)^2+(\gamma_-)^2]/Fz_+$. We derive the non-dimensional form of the concentrations from charge saturation, viz. $\tilde{\varrho} = (c_+\nu - c_-\nu)\cdot[(\gamma_+)^2 +$

$(\gamma_-)^2]$. Hence, we define $\tilde{c}_\alpha = c_\alpha \nu[(\gamma_+)^2 + (\gamma_-)^2]$. As consequence, the electroneutral bulk-state in non-dimensional form becomes $\tilde{c}^{\mathrm{b}} = [(\gamma_+)^2 + (\gamma_-)^2]$ and the steric volume constraint becomes $1 = c_+\nu_+ + c_-\nu_- = (\tilde{c}_+\gamma_+ + \tilde{c}_-\gamma_-)/\tilde{c}^{\mathrm{b}}$. The saturation concentration of species "$\alpha^\star$" becomes $\tilde{c}^{\mathrm{sat}} = \tilde{c}^{\mathrm{b}}/\gamma_{\alpha^\star}$. In the case of symmetric ions ($\gamma_\pm = 1/2$), we find $\tilde{c}^{\mathrm{b}} = 1/2$. Note that the prefactor $(\gamma_+)^2 + (\gamma_-)^2$ remains dangling in eq. (S-36) if an alternative gauge for the charge density or the concentrations is used, e.g. $c_\alpha \nu_\alpha$ or $c_\alpha \nu$.

This yields non-dimensionalized electrostatic fields $\tilde{\boldsymbol{D}} = a^3 \tilde{c}^{\mathrm{b}} \boldsymbol{D}/L_{\mathrm{D}} e z_+$ and $\tilde{\boldsymbol{E}} = L_{\mathrm{D}} e z_+ \boldsymbol{E}/k_{\mathrm{B}} T$, such that $\tilde{\varrho} = \tilde{\boldsymbol{\nabla}} \tilde{\boldsymbol{D}}$, $\tilde{\boldsymbol{E}} = -\tilde{\boldsymbol{\nabla}} \tilde{\Phi}$, and $\tilde{\boldsymbol{D}} = \tilde{\boldsymbol{E}}$.

The next step is to non-dimensionalize the transport equations. For this purpose, we set $\tilde{\mathcal{J}} = -(1+\chi\tilde{\varrho})\tilde{\boldsymbol{\nabla}}\tilde{\mu}_{\mathrm{IL}}$, where the non-dimensionalized chemical forces $\tilde{\boldsymbol{\nabla}}\tilde{\mu}_{\mathrm{IL}} = 1/RTL_{\mathrm{D}} \cdot \boldsymbol{\nabla}\mu_{\mathrm{IL}}$ are subject to the two descriptions eqs. (3) and (7), see also eq. (15). Here, $\chi = (M_+\gamma_- - M_-\gamma_+)/M_{\mathrm{IL}}\tilde{c}^{\mathrm{b}}$ measures the “asymmetry” of the ion-species. We use these non-dimensional quantities to re-express the transport equation for the charge density. For this purpose, we substitute $\tilde{\varrho}$ and $\tilde{\mu}$ into the transport equation derived in the main text,

$$\frac{\varepsilon_{\mathrm{R}}\varepsilon_0}{\kappa}\partial_t \tilde{\varrho} = -\tilde{\boldsymbol{\nabla}}\left(\tilde{\varrho} \cdot \frac{\varepsilon_{\mathrm{R}}\varepsilon_0}{\kappa L_{\mathrm{D}}}\mathbf{v}\right) + \tilde{\boldsymbol{\nabla}}\left([1 + \chi\tilde{\varrho}]\,\tilde{\boldsymbol{\nabla}}\tilde{\mu}_{\mathrm{IL}}\right). \tag{S-37}$$

This suggests defining gauges for the dynamical quantities $\tilde{t} = \kappa/\varepsilon_{\mathrm{R}}\varepsilon_0 \cdot t$ and $\tilde{\mathbf{v}} = \varepsilon_{\mathrm{R}}\varepsilon_0/\kappa L_{\mathrm{D}} \cdot \mathbf{v}$. Note the influence of the electrolyte conductivity $\kappa$ on these two gauges. Altogether, we find

$$\partial_{\tilde{t}}\tilde{\varrho} = \tilde{\boldsymbol{\nabla}}\left[(1 + \chi\tilde{\varrho})\,\tilde{\boldsymbol{\nabla}}\tilde{\mu}_{\mathrm{IL}}\right] - \chi\tilde{\boldsymbol{\nabla}}\left(\tilde{\varrho}\tilde{\mathbf{v}}\right), \tag{S-38}$$

$$\tilde{\boldsymbol{\nabla}}\tilde{\mathbf{v}} = -\tilde{\boldsymbol{\nabla}}\left[(1 + \chi\tilde{\varrho})\,\tilde{\boldsymbol{\nabla}}\tilde{\mu}_{\mathrm{IL}}\right]. \tag{S-39}$$

Furthermore, from the evaluation of the interaction terms follow directly the energy scales $E_{\mathrm{el}}$ and $E_{\mathrm{th}}$, see eqs. (20) and (21). Again, both energies reproduce the canonical textbook expressions used in the literature for symmetric ion-species, i.e. $E_{\mathrm{th}}|_{\gamma_\pm=0.5} = k_{\mathrm{B}}T$ and $E_{\mathrm{el}}|_{\gamma_\pm=0.5} = (ez_+)^2/4\pi\varepsilon_0\varepsilon_{\mathrm{R}}a$ (see, e.g., Ref. S10). These two energy scales can be used to bring the interaction functional into

non-dimensional form (see eq. (19)),

$$\tilde{\mathcal{F}} = \sqrt{\frac{E_{\mathrm{th}}}{8\pi E_{\mathrm{el}}}} \frac{\mathcal{F}/(N_{\mathrm{A}})^2}{8\pi E_{\mathrm{el}}} = \frac{\mathcal{V}^0}{E_{\mathrm{el}}} \sqrt{\frac{E_{\mathrm{th}}}{E_{\mathrm{el}}}} \exp\left(-2\left[\frac{x\pi}{a}\right]^2\right). \tag{S-40}$$

In addition, the energy scales $E_{\mathrm{th}}$ and $E_{\mathrm{el}}$ also non-dimensionalize the perturbation-modes (see eq. (6)),

$$\tilde{\Gamma}^{2n}_{+-} = \frac{\Gamma^{2n}_{+-}}{E_{\mathrm{th}} a^3 (L_{\mathrm{D}})^{2n} (N_{\mathrm{A}})^2}. \tag{S-41}$$

Finally, we summarize our non-dimensional framework in table S-1, where we state all relevant quantities.

**Table S-1: Summary of non-dimensional quantities.**

| Quantity | Dimension | Non-dimensional |
|---|---|---|
| Electrolyte electric potential | $[\Phi] = \mathrm{kg\,m^2\,A^{-1}\,s^{-3}}$ | $\tilde{\Phi} = \Phi \cdot F z_+ / RT$ |
| Electroneutral bulk concentration | $\left[c^{\mathrm{b}}\right] = \mathrm{mol\,m^{-3}}$ | $\tilde{c}^{\mathrm{b}} = (\gamma_+)^2 + (\gamma_-)^2$ |
| Concentration | $[c_\alpha] = \mathrm{mol\,m^{-3}}$ | $\tilde{c}_\alpha = c_\alpha \cdot \nu \tilde{c}^{\mathrm{b}}$ |
| Charge density | $[\varrho] = \mathrm{A\,s\,m^{-3}}$ | $\tilde{\varrho} = \varrho \cdot \nu \tilde{c}^{\mathrm{b}} / F z_+$ |
| Position from electrode | $[x] = \mathrm{m}$ | $\tilde{x} = x / L_{\mathrm{D}}$ |
| Gradient | $[\boldsymbol{\nabla}] = \mathrm{m^{-1}}$ | $\tilde{\boldsymbol{\nabla}} = \boldsymbol{\nabla} \cdot L_{\mathrm{D}}$ |
| Time | $[t] = \mathrm{s}$ | $\tilde{t} = t \cdot \kappa / \varepsilon_0 \varepsilon_{\mathrm{R}}$ |
| Velocity | $[\mathbf{v}] = \mathrm{m\,s^{-1}}$ | $\tilde{\mathbf{v}} = \mathbf{v} \cdot \varepsilon_0 \varepsilon_{\mathrm{R}} / L_{\mathrm{D}} \kappa \chi$ |
| Electric field | $[\boldsymbol{E}] = \mathrm{kg\,m\,A^{-1}\,s^{-3}}$ | $\tilde{\boldsymbol{E}} = \boldsymbol{E} \cdot L_{\mathrm{D}} e z_+ / k_{\mathrm{B}} T$ |
| Dielectric displacement | $[\boldsymbol{D}] = \mathrm{A\,s\,m^{-2}}$ | $\tilde{\boldsymbol{D}} = \boldsymbol{D} \cdot a \tilde{c}^{\mathrm{b}} / L_{\mathrm{D}} e z_+$ |
| Chemical potential | $[\mu_\alpha] = \mathrm{kg\,m^2\,mol^{-1}\,s^{-2}}$ | $\tilde{\mu}_\alpha = \mu_\alpha / RT$ |

# S-3 Binary Ionic Liquid

## S-3.1 Interaction contribution to the chemical forces: Integral Form

In this section, we derive the stationary state equation for the integral description, see eq. (26). For this purpose, we insert eq. (3) into eq. (15),

$$\gamma_+ \boldsymbol{\nabla} \frac{\delta F^{\mathrm{int}}}{\delta c_-} - \gamma_- \boldsymbol{\nabla} \frac{\delta F^{\mathrm{int}}}{\delta c_+} = \frac{1 - 2\gamma_-/\gamma_+}{\nu} \boldsymbol{\nabla}_{\mathbf{x}} \int \mathrm{d}^3 y\, \mathcal{F}_{12}(|\mathbf{x}-\mathbf{y}|) + \frac{2\gamma_+\gamma_-}{F z_+} \boldsymbol{\nabla}_{\mathbf{x}} \int \mathrm{d}^3 y\, \mathcal{F}_{12}(|\mathbf{x}-\mathbf{y}|) \varrho(\mathbf{y}). \tag{S-42}$$

Here, we used labels $\mathbf{x}$ in the derivative operator, to indicate the varied position-variable. However, we make use of symmetry arguments to simplify this expression.

**Lemma 1** *If the interaction potential is spherically symmetric, then the first term on the right side of eq.* (S-42) *vanishes,* $\boldsymbol{\nabla}_{\mathbf{x}} \int \mathrm{d}^3 y\, \mathcal{F}_{12}(|\mathbf{x}-\mathbf{y}|) = 0$.

**Proof:** We make a coordinate transformation to spherical coordinates. Let $r = (|\mathbf{x}-\mathbf{y}|)$ denote the radial coordinate, where, without loss of generality, we choose $\mathbf{x} = 0$. The radial vector is defined by $\boldsymbol{r} = r \cdot \hat{\boldsymbol{e}}_{\boldsymbol{r}} = r \cdot (\sin\theta\cos\phi, \cos\theta\sin\phi, \cos\theta)^T$. The angular coordinates are comprised by the element $\mathrm{d}\Omega = \sin\theta \cdot \mathrm{d}\theta\mathrm{d}\phi$. Thus, we find

$$\boldsymbol{\nabla}_{\mathbf{x}} \int \mathrm{d}^3 y\, \mathcal{F}_{12}(|\mathbf{x}-\mathbf{y}|) = -\int \mathrm{d}r\, \frac{\mathcal{F}'_{12}(r)}{r} \iint \mathrm{d}\Omega\, \boldsymbol{r}, \tag{S-43}$$

where, we used the notation $\mathcal{F}'_{12} = \partial\mathcal{F}_{12}/\partial r$. However, it is easy to show that $\iint \mathrm{d}\Omega\, \boldsymbol{r} = r \cdot \iint \mathrm{d}\Omega\, \hat{\boldsymbol{e}}_{\boldsymbol{r}} = 0$, which completes the proof □

For the rest of this discussion, we restrict to the case of one spatial dimension. Thus, $\nabla = \partial/\partial x$, and eq. (S-42) becomes

$$\gamma_+ \boldsymbol{\nabla} \frac{\delta F^{\mathrm{int}}}{\delta c_-} - \gamma_- \boldsymbol{\nabla} \frac{\delta F^{\mathrm{int}}}{\delta c_+} = \frac{2\gamma_+\gamma_-}{F z_+} \boldsymbol{\nabla}_{\mathbf{x}} \int \mathrm{d}^3 y\, \mathcal{F}_{12}(|\mathbf{x}-\mathbf{y}|)\varrho(\mathbf{y}). \tag{S-44}$$

Next, we integrate both over the interval $\mathcal{I} = [x; L_{\mathrm{DL}}]$, where $L_{\mathrm{DL}}$ denotes the width of the ED, using electroneutral boundary conditions,

$$\Phi'(L_{\mathrm{DL}}) = 0, \quad \Phi(L_{\mathrm{DL}}) = 0, \quad \varrho(L_{\mathrm{DL}}) = 0, \quad c_\alpha(L_{\mathrm{DL}}) = 1/\nu = c^{\mathrm{b}}. \tag{S-45}$$

We use these BCs and integrate the interaction-term, yielding $\int_x^{L_{\mathrm{DL}}} \mathrm{d}\hat{x}\, \nabla \int_0^{L_{\mathrm{DL}}} \mathrm{d}y \mathcal{F}_{12}(|\hat{x}-y|)\varrho(y) = \int_0^{L_{\mathrm{DL}}} \mathrm{d}y\, \mathcal{F}_{12}(|L_{\mathrm{DL}}-y|)\varrho(y) - \int_0^{L_{\mathrm{DL}}} \mathrm{d}y\, \mathcal{F}_{12}(|x-y|)\varrho(y)$. The first term on the right side can be neglected if the potential $\mathcal{F}_{12}$ is of short range, and if we assume the electroneutral BC for the charge-density $\lim_{x\to L_{\mathrm{DL}}} \varrho(x) = 0$. The non-dimensional form follows straightforwardly.

## S-3.2 Special Case: Symmetric Ion species

In this section, we discuss the case of completely symmetric ion-species, *i.e.* have equal molar masses and volumes. First, we restate the dynamic transport equations,

$$\partial_{\tilde{t}}\tilde{\varrho} = \tilde{\nabla}\left[(1+\chi\tilde{\varrho})\,\tilde{\nabla}\tilde{\mu}_{\rm IL}\right] - \chi\tilde{\nabla}\left(\tilde{\varrho}\tilde{\mathbf{v}}\right), \quad \tilde{\nabla}\tilde{\mathbf{v}} = -\tilde{\nabla}\left[(1+\chi\tilde{\varrho})\,\tilde{\nabla}\tilde{\mu}_{\rm IL}\right]. \tag{S-46}$$

In this case, the asymmetry factor appearing above becomes trivial, $\chi = 0$. Hence, system of transport equation becomes

$$\partial_{\tilde{t}}\tilde{\varrho} = -\tilde{\nabla}\tilde{\mathbf{v}} = \tilde{\nabla}^2\tilde{\mu}_{\rm IL}, \tag{S-47}$$

where the chemical forces are $\tilde{\nabla}\tilde{\mu}_{\rm IL} = -\tilde{\nabla}(\tilde{\Phi} - \gamma_+\ln[\tilde{c}_-/\tilde{c}^{\rm b}] + \gamma_-\ln[\tilde{c}_+/\tilde{c}^{\rm b}] - \gamma_+/RT\cdot\delta F^{\rm int}/\delta c_- + \gamma_-/RT\cdot\delta F^{\rm int}/\delta c_+)$. We substitute the Poisson equation for the left side of eq. (S-47), $\tilde{\varrho} = -\tilde{\nabla}^2\tilde{\Phi}$, which yields $\tilde{\nabla}^2(\partial_{\tilde{t}}\tilde{\Phi} + \tilde{\mu}_{\rm IL}) = 0$. Upon using electroneutral boundary conditions, this can be integrated twice such that the system is completely described by

$$\partial_{\tilde{t}}\tilde{\Phi} = -\tilde{\mu}_{\rm IL}, \tag{S-48}$$

where the chemical potential can be expressed either using the integral description (see right side of eq. (26)), or the gradient description (see right side of eq. (25)).

Apparently, the stationary state equation for symmetric ion species, $\mu_{\rm IL} = 0$, equals exactly the stationary state equation of non-symmetric ion-species, see eqs. (25) and (26).

## S-3.3 Mean Steric Effect: Charge Saturation

In this section, we discuss the "bulk"-description for the EDL ($\mathcal{V}^0 = 0$), outlined in section III B. In sections S-3.3.1 and S-3.3.2, we discuss the charge comprised in the EDL, and the corresponding differential capacitance. In addition, we show how the EDL-width depends upon ion-asymmetry in section S-3.3.1. Next, we discuss the general case of symmetric ion-species in section S-3.3.3.

#### S-3.3.1 Asymptotic Analysis for Small Potentials: EDL Charge and Differential Capacitance

Here, we consider the bulk-description for the EDL ($\mathcal{V}^0 = 0$) in the electroneutral approximation outlined in section III B 1.

In the main text (see eq. (35)), we found that the screening profile for the electric potential exhibits an exponential shape for the region far away from the interface. According to this description, the width of the EDL is determined by the inverse Debye-length via the damping parameter $k = 1/L_\mathrm{D}$.

First, we discuss how the width of the EDL depends upon the asymmetry of the ion-sizes. For this purpose, we introduce the asymmetry-parameter $\xi = \gamma_+/\gamma_-$, such that the inverse of eq. (17) becomes

$$k(\xi) = \sqrt{\frac{(ez_+)^2}{k_\mathrm{B}T\varepsilon_0\varepsilon_\mathrm{R}a^3\tilde{c}^\mathrm{b}}} \cdot \frac{1+\xi}{\sqrt{1+\xi^2}}. \tag{S-49}$$

Apparently, $k(\xi)$ has a global minimum at $\xi = 1$, *i.e.* the EDL-width is maximal for ion-species of equal size.

Next, we discuss the charge comprised in the EDL, and the differential capacitance. The cumulative charge from the electroneutral bulk up to position $x$ in the electrolyte, $\mathcal{Q}(x)$, is determined by the electric field,

$$\mathcal{Q}(x) = \int_x^{L_\mathrm{EDL}} \mathrm{d}y\, \varrho(y) = -\varepsilon_0\varepsilon_\mathrm{R} \int_x^{L_\mathrm{EDL}} \mathrm{d}y\, \Phi''(y) = \varepsilon_0\varepsilon_\mathrm{R}\Phi'(x) = -\varepsilon_0\varepsilon_\mathrm{R}\Phi(x)/L_\mathrm{D}. \tag{S-50}$$

Here we used the electroneutral boundary condition $\Phi' L_\mathrm{EDL} = 0$. The total surface-charge-density comprised in the EDL is thus given by the boundary condition for the electric field at the interface,

$$\mathcal{Q}^\mathrm{tot} = \mathcal{Q}(0) = -\varepsilon_0\varepsilon_\mathrm{R}\Delta\phi/L_\mathrm{D}, \tag{S-51}$$

whereas the corresponding differential capacitance is

$$\frac{\mathrm{d}\mathcal{Q}^{\mathrm{tot}}}{\mathrm{d}(\varDelta\phi)} = -\varepsilon_0\varepsilon_{\mathrm{R}}/L_{\mathrm{D}}. \tag{S-52}$$

### S-3.3.2 Asymptotic Analysis for Large Potentials: EDL Charge and Differential Capacitance

Here, we discuss the bulk-description for the EDL at regions close to the interface, see section III B 2. There, we found analytical solutions for $\tilde{\varPhi}$ and $\tilde{\varrho}$, see eqs. (36) and (38). Here, we state the dimensional form of the solution for the electric potential,

$$\varPhi(x) = \varDelta\phi \cdot (1 - x/L_{\mathrm{EDL}})^2\,, \tag{S-53}$$

from which we calculate the charge comprised in the EDL, and the corresponding differential capacitance.

The cumulative EDL-charge comprised in the electrolyte region from the electroneutral bulk up to position $x$, $\mathcal{Q}(x)$, is determined by

$$\mathcal{Q}(x) = \int_x^{L_{\mathrm{EDL}}} \mathrm{d}y\, \varrho(y) = -\varepsilon_0\varepsilon_{\mathrm{R}} \int_x^{L_{\mathrm{EDL}}} \mathrm{d}y\, \varPhi''(y) = -\frac{2\varepsilon_0\varepsilon_{\mathrm{R}}\varDelta\varPhi}{L_{\mathrm{EDL}}} \cdot (1 - x/L_{\mathrm{EDL}})\,. \tag{S-54}$$

Above, we used the Poisson equation ($\varrho = -\varepsilon_0\varepsilon_{\mathrm{R}}\varPhi''$), electroneutral boundary conditions for the electric field, and the solution eq. (S-53). From this cumulative charge follows the total surface-charge-density $\mathcal{Q}^{\mathrm{tot}}$, comprised in the complete EDL, and the corresponding differential capacitance,

$$\mathcal{Q}^{\mathrm{tot}}(a, \varepsilon_{\mathrm{R}}, T, \varDelta\phi, \gamma_\pm) = \mathcal{Q}(0) = -\frac{2\varepsilon_0\varepsilon_{\mathrm{R}}\varDelta\phi}{L_{\mathrm{EDL}}} = -\mathrm{sign}\,(\varDelta\phi)\sqrt{\frac{2|\varDelta\phi|\varepsilon_0\varepsilon_{\mathrm{R}}(ez_+)^2}{k_{\mathrm{B}}Ta^3\gamma_{\alpha^*}}}, \tag{S-55}$$

$$\frac{\mathrm{d}\mathcal{Q}^{\mathrm{tot}}}{\mathrm{d}(\varDelta\phi)} = -\sqrt{\frac{\varepsilon_0\varepsilon_{\mathrm{R}}(ez_+)^2}{2k_{\mathrm{B}}Ta^3\gamma_{\alpha^*}|\varDelta\phi|}}. \tag{S-56}$$

### S-3.3.3 Mean Volume Effect: Symmetric Ions

Here, we discuss the bulk-description for the EDL eq. (31) in the special case where the ion-species have the same molar volume, *i.e.* $\gamma_\pm = \tilde{c}^{\mathrm{b}} = 1/2$. In this case, eq. (31) can be exponentiated such that $\tilde{c}_- = \tilde{c}_+ \cdot \exp(2\tilde{\Phi})$. Using charge conservation, $\tilde{\varrho} = \tilde{c}_+ - \tilde{c}_-$ and $\tilde{c}_- = (1-\tilde{\varrho})/2$, we derive an expression for the charge density as function of the electric potential,

$$\tilde{\varrho}(\tilde{\Phi}) = \frac{1-\exp(2\tilde{\Phi})}{1+\exp(2\tilde{\Phi})} = -\tanh(\tilde{\Phi}) \tag{S-57}$$

Next, we derive an equation for the electric field as function of the electric potential. For this purpose, we substitute the Poisson equation ($\tilde{\varrho} = -\tilde{\Phi}''$ for the left side above, and multiply both sides by $2\tilde{\Phi}'$. We integrate both sides over the interval $[x; L_{\mathrm{DL}}]$, where we make use of electroneutral BCs (see eq. (S-45)), and evaluate the relation $2\tilde{\Phi}'\tilde{\Phi}'' = \boldsymbol{\nabla}[(\tilde{\Phi}')^2] = \mathrm{d}[(\tilde{\Phi}')^2]$. Thereby, we find

$$\tilde{\boldsymbol{E}} = -\tilde{\Phi}' = \mathrm{sign}\,(\Delta\phi)\,\sqrt{2\ln[\cosh(\tilde{\Phi})]}, \tag{S-58}$$

$$\mathcal{Q}^{\mathrm{tot}} = -\mathrm{sign}\,(\Delta\phi)\,\frac{k_{\mathrm{B}}T\varepsilon_0\varepsilon_{\mathrm{R}}}{L_{\mathrm{D}}e|z_+|}\,\sqrt{2\ln[\cosh(\tilde{\Phi})]}. \tag{S-59}$$

## S-3.4 Non-Local Interactions: Charge Oscillations

In this section, we discuss various aspects of our EDL-description which takes account for non-local molecular interactions ($\mathcal{V}^0 \neq 0$). In section S-3.4.1, we derive the first two the perturbation modes appearing in the gradient expansion of the interaction functional. Next, in section S-3.4.2 we present a detailed proof for the existence of three different screening phases. We probe these screening phases by discussing limiting cases for the interaction energy in section S-3.4.3. In addition, we probe the emergence of screening phases when only the trivial perturbation mode is considered, see section S-3.4.4, and when only the linear order is considered, see section S-3.4.5.

### S-3.4.1 Perturbation Modes

In this section, we calculate the first two perturbation modes, $\Gamma^0_\pm$ and $\Gamma^2_\pm$ (eqs. (10) and (11)) appearing in the gradient approximation of the Gauss-Ansatz (see eq. (9)) for the interaction functional.

As first step, we make use of the spherical symmetry of the interaction potential, which implies that

$$\Gamma^{2n}_{\alpha\beta} = \frac{1}{(2n)!} \cdot \int \mathrm{d}x^3\, \mathcal{F}_{\alpha\beta}(|x|) x^{2n} = \frac{4\pi}{(2n)!} \cdot \int \mathrm{d}r\, \mathcal{F}_{\alpha\beta}(r) \cdot r^{2(n+1)} \tag{S-60}$$

However, this integral can be solved analytically when the shape of the interaction potential is determined by a Gauss profile,

$$4\pi \int \mathrm{d}r\, \exp\left[-\left(\frac{r}{\ell_{\mathrm{int}}}\right)^2\right] \cdot r^{2(n+1)} = 2\pi \cdot (\ell_{\mathrm{int}})^{2n+3} \cdot \Gamma\left(\frac{2n+3}{2}\right). \tag{S-61}$$

Here, $\Gamma\left(\frac{n}{2}\right)$ is the Gamma-function, where, *e.g.*, $\Gamma\left(\frac{5}{2}\right) = 3/2 \cdot \Gamma\left(\frac{3}{2}\right) = 3/2 \cdot \sqrt{\pi}/2$. For the correlation length $\ell_{\mathrm{int}} = a/\pi\sqrt{2}$ (see main text), we find

$$\int \mathrm{d}x^3\, \exp\left[-\left(\frac{x}{\ell_{\mathrm{int}}}\right)^2\right] = \left(\frac{a}{\sqrt{2\pi}}\right)^3, \tag{S-62}$$

and

$$\frac{1}{(2)!} \int \mathrm{d}x^3\, \exp\left[-\left(\frac{x}{\ell_{\mathrm{int}}}\right)^2\right] \cdot x^2 = \frac{1}{2} \cdot \left(\frac{a}{\sqrt{2}\pi}\right)^2 \left(\frac{a}{\sqrt{2\pi}}\right)^3. \tag{S-63}$$

The two perturbation modes eqs. (10) and (11) follow directly from the results eqs. (S-62) and (S-63).

### S-3.4.2 Analysis of the Phase Space of Screening Profiles

In the main text (see section IV A 2), we show that the signature of eigenvalues $\tilde{\alpha}_{1,2}$ determines the phase space of screening profiles. Here, we present a detailed proof for the emergence of three screening phases.

To address this goal, we make a thorough analytical investigation of the root $\mathcal{W}$ appearing in the eigenvalue-equation derived in the main text (see eq. (41)). For completeness, we restate it

here,

$$\tilde{\alpha}_{1,2} = -\pi E_{\mathrm{th}}/4E_{\mathrm{el}} \cdot [1 - E_{\mathrm{th}}/\mathcal{V}^0 \mp \sqrt{(1 - E_{\mathrm{th}}/\mathcal{V}^0)^2 - 8E_{\mathrm{el}}/\pi\mathcal{V}^0}]. \tag{S-64}$$

The sign of the root $\mathcal{W}(\mathcal{V}^0) = (1 - E_{\mathrm{th}}/\mathcal{V}^0)^2 - 8E_{\mathrm{el}}/\mathcal{V}^0\pi$ determines whether the quantities $\tilde{\alpha}_{1,2}$ are complex-valued or real-valued. Thus, in order to identify the parameter space at which the root is positive and negative, we first derive the parameters

$$\mathcal{V}^0_{\pm} = E_{\mathrm{th}} + 4E_{\mathrm{el}}/\pi \pm \sqrt{8E_{\mathrm{el}}/\pi\,(2E_{\mathrm{el}}/\pi + E_{\mathrm{th}})}, \tag{S-65}$$

where the root is exactly zero, *i.e.* $\mathcal{W}(\mathcal{V}^0_{\pm}) = 0$. The next step is to conduct a complete curve analysis. However, we first prove some Lemmata, which are useful to address this goal. Eventually, this leads to the principal finding of this curve analysis, comprised in Theorem 1.

**Lemma 2** $E_{\mathrm{th}} + 4E_{\mathrm{el}}/\pi < \mathcal{V}^0_{+} \leq 8E_{\mathrm{el}}/\pi + E_{\mathrm{th}} + 2\sqrt{2E_{\mathrm{el}}E_{\mathrm{th}}/\pi}$.

**Proof:** The left side of the inequality follows trivially from the definitions of $\mathcal{V}^0_{\pm}$, see eq. (S-65). The inequality appearing on the right side above follows from the triangle-inequality,

$$\sqrt{8E_{\mathrm{el}}/\pi\,(2E_{\mathrm{el}}/\pi + E_{\mathrm{th}})} \leq 4E_{\mathrm{el}}/\pi + \sqrt{8E_{\mathrm{el}}E_{\mathrm{th}}/\pi}.$$

This completes the proof. □

**Lemma 3** *Both roots* $\mathcal{V}^0_{\pm}$ *are positive.*

**Proof:** Positivity of $\mathcal{V}^0_{+}$ is trivial. In order to prove the claim for $\mathcal{V}^0_{-}$, we use the alternative expression

$$\mathcal{V}^0_{-} = 4E_{\mathrm{el}}/\pi \cdot \left(1 + \pi E_{\mathrm{th}}E_{\mathrm{el}}/4 - \sqrt{1 + \pi E_{\mathrm{th}}E_{\mathrm{el}}/2}\right). \tag{S-66}$$

Next, we use that the relation $1 + x < 1 + x + x^2/4$, valid for any $x > 0$, which implies that $\sqrt{1+x} < 1 + x/2$. Thus, we can give an upper bound for the root $\sqrt{1 + \pi E_{\mathrm{th}}E_{\mathrm{el}}/2} < 1 + \pi E_{\mathrm{th}}E_{\mathrm{el}}/4$, such that the bracked term on the right side of eq. (S-66) is positive and not zero. This completes the proof. □

Next, we examine the properties of $\mathcal{W}$ via the determination of it's extrema. The derivative

$$\mathcal{W}' = \frac{d\mathcal{W}}{d\mathcal{V}^0} = \cdot \left(\mathcal{V}^0 \cdot [2E_{\mathrm{th}} + 8E_{\mathrm{el}}/\pi] - 2E_{\mathrm{th}}^2\right)/(\mathcal{V}^0)^3, \tag{S-67}$$

is zero exactly at

$$\mathcal{V}^0_\square = \frac{E_{\mathrm{th}}}{1 + 4E_{\mathrm{el}}E_{\mathrm{th}}/\pi}. \tag{S-68}$$

**Lemma 4** $\mathcal{V}^0_- < \mathcal{V}^0_\square < \mathcal{V}^0_+$.

**Proof:** Apparently, from eq. (S-68) follows directly that $\mathcal{V}^0_\square < E_{\mathrm{th}}$. Hence, due to Lemma 2, $\mathcal{V}^0_\square < \mathcal{V}^0_+$. In order to prove the second claim of the Lemma, we expand $\mathcal{V}^0_-$ in $\mathcal{V}^0_\square$,

$$\mathcal{V}^0_- = \mathcal{V}^0_\square \cdot \left(1 + \frac{4E_{\mathrm{el}}}{\pi E_{\mathrm{th}}}\left[1 + \left(1 + \frac{4E_{\mathrm{el}}}{\pi E_{\mathrm{th}}}\right) \cdot \left(1 - \sqrt{1 + \pi E_{\mathrm{th}}/2 \cdot E_{\mathrm{el}}}\right)\right]\right). \tag{S-69}$$

The square-root on the right side is larger than one. Simple algebra then shows that the outermost bracked term is smaller than one, which completes the proof. □

**Lemma 5** $\mathcal{V}^0_- < E_{\mathrm{th}}$.

**Proof:** Apparently, eq. (S-68) implies that $\mathcal{V}^0_\square < E_{\mathrm{th}}$. Thus, due to transitivity, Lemma 4 completes the proof. □

**Lemma 6** $\mathcal{W}(\mathcal{V}^0_\square) < 0$.

**Proof:** Insertion of eq. (S-68) into $\mathcal{W}$ yields $\mathcal{W}(\mathcal{V}^0_\square) = -(4 + 8E_{\mathrm{el}}E_{\mathrm{th}}/\pi) \cdot 2E_{\mathrm{el}}E_{\mathrm{th}}/\pi$. All prefactors are positive, which completes the proof. □

As consequence, the roots $\mathcal{V}^0_\pm$ define three regions along the direction of increasing $\mathcal{V}^0$: *Region I* is defined by $0 < \mathcal{V}^0 < \mathcal{V}^0_-$, *region II* is defined by $\mathcal{V}^0_- < \mathcal{V}^0 < \mathcal{V}^0_+$, and *region III* is defined by $\mathcal{V}^0_+ < \mathcal{V}^0$.

**Lemma 7** *The root $\mathcal{W}$ is positive in regions I&III, and negative in region II.*

**Proof:** This follows from Lemma 6, together with the relations implied by Lemma 4. $\square$

**Lemma 8** *In regions I&III,* $0 < 8E_{\mathrm{el}}\mathcal{V}^0/\pi(E_{\mathrm{th}} - \mathcal{V}^0)^2 < 1$.

**Proof:** In these regions, $\mathcal{W} > 0$. Hence, $(1 - E_{\mathrm{th}}/\mathcal{V}^0)^2 > 8E_{\mathrm{el}}/\pi\mathcal{V}^0$. This completes the proof. $\square$

We use the inequality appearing in lemma 8 to check for the sign of the eigenvalues. For this purpose, we write eq. (41) in the form

$$\tilde{\alpha}_{1,2} = -\frac{\pi}{4} \cdot \frac{E_{\mathrm{th}}}{E_{\mathrm{el}}} \cdot \left(1 - \frac{E_{\mathrm{th}}}{\mathcal{V}^0}\right) \cdot \left[1 \mp \sqrt{1 - 8E_{\mathrm{el}}\mathcal{V}^0/\pi(E_{\mathrm{th}} - \mathcal{V}^0)^2}\right]. \tag{S-70}$$

**Lemma 9** *All eigenvalues are real and positive in region I, i.e.* $0 < \tilde{\alpha}_{1,2}(\mathcal{V}^0 < \mathcal{V}^0_-) \in \mathbb{R}$.

**Proof:** Let $\mathcal{V}^0 < \mathcal{V}^0_-$. Thus, $\tilde{\alpha}_{1,2} \in \mathbb{R}$, since $\mathcal{W} > 0$ according to Lemma 7. Due to Lemma 8, the last factor in eq. (S-70) is always positive in this region. Thus, the sign of the eigenvalues is determined by the relative magnitude of $\mathcal{V}^0$ and $E_{\mathrm{th}}$. However, due to Lemma 5, $\mathcal{V}^0 < E_{\mathrm{th}}$, in this region, such that $1 - E_{\mathrm{th}}/\mathcal{V}^0 < 0$. This completes the proof. $\square$

**Lemma 10** *All eigenvalues are real and negative in region III, i.e.* $0 > \tilde{\alpha}_{1,2}(\mathcal{V}^0_+ < \mathcal{V}^0) \in \mathbb{R}$.

**Proof:** We apply the same argument as in the proof for Lemma 8. Again, the signs of the eigenvalues are determined by the ratio $E_{\mathrm{th}}/\mathcal{V}^0$. However, in *region III*, $E_{\mathrm{th}} < \mathcal{V}^0$, which completes the proof. $\square$

**Lemma 11** *All eigenvalues are complex in region II, i.e.* $\tilde{\alpha}_{1,2}(\mathcal{V}^0_- < \mathcal{V}^0 < \mathcal{V}^0_+) \in \mathbb{R} \times i \cdot \mathbb{R}$.

**Proof:** Due to Lemma 7, $\sqrt{\mathcal{W}} \in i \cdot \mathbb{R}$. Thus, according to eq. (S-70), the eigenvalues have the form

$$\tilde{\alpha}_{1,2} = \frac{\pi}{4} \cdot \frac{E_{\mathrm{th}}}{E_{\mathrm{el}}} \left(\frac{E_{\mathrm{th}}}{\mathcal{V}^0} - 1\right) \cdot (1 \pm i \cdot w)\,, \tag{S-71}$$

where $w = \mathrm{Im}(\sqrt{\mathcal{W}})$. This completes the proof. $\square$

Next, we examine the eigenvalues at exactly the phase boundaries.

**Lemma 12** *$0 > \tilde{\alpha}_{1,2}(\mathcal{V}^0_+) \in \mathbb{R}$, and $0 < \tilde{\alpha}_{1,2}(\mathcal{V}^0_-) \in \mathbb{R}$.*

**Proof:** By construction, $\mathcal{W}(\mathcal{V}^0_\pm) = 0$, such that the eigenvalue-equation is real-valued, and becomes

$$\tilde{\alpha}_{1,2}(\mathcal{V}^0_\pm) = \frac{\pi}{4} \cdot \frac{E_{\text{th}}}{E_{\text{el}}} \left( \frac{E_{\text{th}}}{\mathcal{V}^0} - 1 \right). \tag{S-72}$$

Lemmata 2 and 5 then complete the proof. □

With the help of the previous Lemmata, we state the principal finding of this section.

**Theorem 1** *The phase-space of screening profiles is threefold:*

*Region I) $\mathcal{V}^0 \leq \mathcal{V}^0_-$: exponentially damped screening profile;*

*Region II) $\mathcal{V}^0_- \leq \mathcal{V}^0 \leq \mathcal{V}^0_+$: exponentially damped, oscillatory screening profile;*

*Region III) $\mathcal{V}^0_+ \leq \mathcal{V}^0$: undamped oscillatory screening profile;*

**Proof:** The screening parameter which determines the profile of the solution eq. (39) is defined by $\tilde{k}^{\tilde{\alpha}_{1,2}} = \pm\sqrt{\tilde{\alpha}_{1,2}}$. Thus, the profile depends upon the number-field of $\tilde{\alpha}_{1,2}$. Using Lemmata 9-12 completes the proof. □

### S-3.4.3 Limiting Cases

In this section we examine the limiting cases of indefinitely large values of $\mathcal{V}^0$, and of vanishing small values of $\mathcal{V}^0$.

Theorem 1 implies that the limit $\mathcal{V}^0 \to \infty$ yields undamped oscillations. In particular, the evaluation of eq. (41) in this limit yields $\lim_{\mathcal{V}^0\to\infty} \tilde{\alpha}_{1,2} = -\pi E_{\text{th}}/2E_{\text{el}}(1 \mp 1)$, such that

$$\lim_{\mathcal{V}^0\to\infty} \tilde{k}^{\tilde{\alpha}_2} = \pm \lim_{\mathcal{V}^0\to\infty} \sqrt{\tilde{\alpha}_2} = \pm i \cdot \sqrt{\pi E_{\text{th}}/2E_{\text{el}}} = \pm i 2\pi/a \tag{S-73}$$

and

$$\lim_{\mathcal{V}^0\to\infty} \tilde{k}^{\tilde{\alpha}_1} = \pm \lim_{\mathcal{V}^0\to\infty} \sqrt{\tilde{\alpha}_1} = 0. \tag{S-74}$$

Here, we used eq. (22). Apparently, the limit eq. (S-74) renders unphysical, as it implies a constant screening profile. In contrast, eq. (S-73) reproduces the correlation between the frequency of the oscillations and the ion-sizes stated in the main text (see eq. (48)).

It remains to investigate the limit of vanishing interactions, $\mathcal{V}^0 \to 0$. For this purpose, we write the eigenvalue-equation eq. (41) in the form

$$\tilde{\alpha}_{1,2} = -\frac{\pi}{4} \cdot \frac{E_{\mathrm{th}}}{E_{\mathrm{el}}} \cdot \frac{1}{\mathcal{V}^0} \left[ \mathcal{V}^0 - E_{\mathrm{th}} \mp \sqrt{(\mathcal{V}^0 - E_{\mathrm{th}})^2 - 8E_{\mathrm{el}}\mathcal{V}^0/\pi} \right], \tag{S-75}$$

and Taylor-expand the square-root for small values $\mathcal{V}^0$. This yields, up to the first order in $\mathcal{V}^0$,

$$\sqrt{(\mathcal{V}^0 - E_{\mathrm{th}})^2 - 8E_{\mathrm{el}}\mathcal{V}^0/\pi} \approx E_{\mathrm{th}} - (1 + 4E_{\mathrm{el}}/\pi E_{\mathrm{th}}) \cdot \mathcal{V}^0. \tag{S-76}$$

Thus, in this approximation, we get find that $\lim_{\mathcal{V}^0 \to 0} \tilde{\alpha}_{1,2}$ converges towards one finite limiting parameter, and one un-physical parameter

$$\lim_{\mathcal{V}^0 \to 0} \tilde{k}^{\tilde{\alpha}_1} \to \pm\infty, \tag{S-77}$$

$$\lim_{\mathcal{V}^0 \to 0} \tilde{k}^{\tilde{\lambda}_2} = 1. \tag{S-78}$$

Thus, we recover the EDL-width as predicted by the analytical discussion in section III B 1, see eqs. (33) to (35). This highlights that the interaction-theory transitions into the bulk theory in the limit of vanishing interaction strengths.

### S-3.4.4 Trivial Order Expansion

In this section, we consider only the trivial order ($n = 0$) in the gradient description. This reduces the expansion of the dielectric operator eq. (30) to a scalar parameter, $\hat{\varepsilon}_{\mathrm{R}} \to \varepsilon_{\mathrm{R}}^{(n=0)} = 1 - \tilde{\Gamma}^0_{+-} = 1 - \mathcal{V}^0/E_{\mathrm{th}}$. Thus, the corresponding transport equation for the charge density (see eq. (28)) reads

$$\tilde{\Phi} = \varepsilon_{\mathrm{R}}^{(n=0)} \cdot \tilde{\Phi}'' = \left(1 - \mathcal{V}^0/E_{\mathrm{th}}\right) \cdot \tilde{\Phi}''. \tag{S-79}$$

Depending upon the sign of $\varepsilon_{\mathrm{R}}^{(n=0)}$ the exponential solution to this differential equation exhibits either an exponentially damped profile ($\varepsilon_{\mathrm{R}}^{(n=0)} < 0$, *i.e.* $E_{\mathrm{th}} < \mathcal{V}^0$), or an oscillatory (undamped) profile ($\varepsilon_{\mathrm{R}}^{(n=0)} > 0$, *i.e.* $E_{\mathrm{th}} > \mathcal{V}^0$). As consequence, in this trivial order, the phase space is reduced to two distinct screening phases, where the corresponding phase boundary is determined by $\mathcal{V}^0_{\mathrm{crit}} = E_{\mathrm{th}}$. Apparently, the thermal energy and the interaction energy constitute the relevant energy scales for the screening profile, whereas the electrostatic energy has no influence. Here, we assume that both energy scales $\mathcal{V}^0$ and $E_{\mathrm{th}}$ are positive. As consequence, the correction $\tilde{\Gamma}$ to the electrostatic parameter $\varepsilon_{\mathrm{R}} = 1$ corresponds to a mitigation of the electrostatic energy. Thus, from an alternative points of view, only $E_{\mathrm{th}}$ and $E_{\mathrm{el}}$ characterize the phase space, where a negative dielectricity yields undamped oscillations.

Next, we shall investigate the influence of the ion-asymmetry on the phase space of screening profiles. For this purpose, we evaluate the phase boundary $\mathcal{V}^0_{\mathrm{crit}}(\xi) = k_{\mathrm{B}}T/2 \cdot (1 + \xi^2)/\xi$. Here, we used the asymmetry parameter $\xi = \gamma_+/\gamma_-$ introduced in section S-3.3.1. It is easy to show that $\mathcal{V}^0_{\mathrm{crit}}$ has a global minimum at $\xi = 1$, *i.e.* for equal molar volumes of the ion-species. Thus, ion-asymmetry is favourable for $E_{\mathrm{th}}$ in the competition between thermal disordering and molecular interactions, and the transition from exponential to oscillatory profiles is shifted to smaller interaction energies for alike molar volume of the ion-species. This highlights the influence of ion-asymmetry on the phase-space. At fixed temperature, the phase boundary becomes minimal for ions of equal size, $\mathrm{d}\mathcal{V}^0_{\mathrm{crit}}/\mathrm{d}\gamma|_{\gamma=1} = 0$. Thus, the larger the discrepancy between the size of the ion-species, the larger the entropic dominance becomes.

Note that if the interaction parameter $\mathcal{V}^0$ is negative, then the phase space reduces to the classical case, where only exponentially damped profiles emerge. This then corresponds to an increased magnitude of the dielectricity $\varepsilon_{\mathrm{R}} = 1 + |\mathcal{V}^0|/E_{\mathrm{th}}$, *i.e.* negative interaction energies contribute to $E_{\mathrm{th}}$ and the effective strength of the electrostatic energy scale increases.

### S-3.4.5 Linear Order Expansion

In this section, we consider the case where only the first order ($n = 1$) contributes to the gradient description. Thus, the resulting dielectric operator becomes $\hat{\varepsilon}_{\rm R} \to \hat{\varepsilon}_{\rm R}^{(n=1)} = 1 - \tilde{\Gamma}^2_{+-}\tilde{\boldsymbol{\nabla}}^2$, where $\tilde{\Gamma}^2_{+-} = 2/\pi \cdot \mathcal{V}^0/E_{\rm th} \cdot E_{\rm el}/E_{\rm th}$ (see eqs. (30) and (S-41)). Hence, the corresponding system of equations (see eqs. (28) and (39)) becomes

$$\begin{pmatrix} \tilde{\varrho}'' \\ \tilde{\Phi}'' \end{pmatrix} = \mathcal{A}^{(n=1)} \cdot \begin{pmatrix} \tilde{\varrho} \\ \tilde{\Phi} \end{pmatrix} = \begin{pmatrix} 1/\tilde{\Gamma}^2_{+-} & 1/\tilde{\Gamma}^2_{+-} \\ -1 & 0 \end{pmatrix} \cdot \begin{pmatrix} \tilde{\varrho} \\ \tilde{\Phi} \end{pmatrix}. \tag{S-80}$$

The solutions to this system of equations are determined by the eigenvalues $\tilde{\alpha}_{1,2}^{(n=1)}$ corresponding to the matrix $\mathcal{A}^{(n=1)}$, which are completely determined by $\tilde{\Gamma}^2_{+-}$, *viz.*

$$\tilde{\alpha}_{1,2} = -\frac{1}{2\tilde{\Gamma}^2_{+-}}\left(1 \mp \sqrt{1 - \tilde{\Gamma}^2_{+-}}\right) = -\frac{\pi}{4} \cdot \frac{E_{\rm th}}{\mathcal{V}^0} \cdot \frac{E_{\rm th}}{E_{\rm el}}\left(1 \mp \sqrt{1 - \frac{8}{\pi}\frac{\mathcal{V}^0}{E_{\rm th}}\frac{E_{\rm el}}{E_{\rm th}}}\right). \tag{S-81}$$

Like in the full expansion comprising the trivial and linear order in the gradient expansion, the zeros of the root $\mathcal{W} = 1 - 8/\pi \cdot \mathcal{V}^0/E_{\rm th} \cdot E_{\rm el}/E_{\rm th}$ determine the sign of the eigenvalue, *i.e.* the phase boundaries. Here, only one such critical value for the interaction strength exists,

$$\mathcal{V}^0_{\rm crit} = E_{\rm th} \cdot \frac{\pi}{8} \cdot \frac{E_{\rm th}}{E_{\rm el}}. \tag{S-82}$$

Thus, only two screening phases exist in this case. For $\mathcal{V}^0 < \mathcal{V}^0_{\rm crit}$, all eigenvalues are positive, which implies that the profiles are exponentially damped. In contrast, if $\mathcal{V}^0_{\rm crit} < \mathcal{V}^0$, the root becomes purely complex, $\sqrt{\mathcal{W}} \in i \cdot \mathbb{R}$. Hence, all eigenvalues have non-vanishing real-/ and imaginary parts, $\tilde{\alpha}_{1,2} \in \mathbb{R} \times i \cdot \mathbb{R}$. This implies damped oscillations.

In particular, if the interaction parameter $\mathcal{V}^0$ is positive, there are no cases where the eigenvalues are real but negative, yielding purely complex wave-numbers $\tilde{k} = \sqrt{\tilde{\alpha}_{1,2}} \in i \cdot \mathbb{R}$. Thus, the case of undamped oscillations does not occur if we take only the first interacting order into account.

Interestingly, for negative values $\mathcal{V}^0 < 0$, the phase-space changes. For such energies $\mathcal{V}^0 =$

$-|\mathcal{V}^0|$, the eigenvalue-equation can be written

$$\tilde{\alpha}_{1,2} = \frac{\pi}{4} \cdot \frac{E_{\text{th}}}{|\mathcal{V}^0|} \cdot \frac{E_{\text{th}}}{E_{\text{el}}} \left( 1 \mp \sqrt{1 + \frac{8}{\pi} \frac{|\mathcal{V}^0|}{E_{\text{th}}} \frac{E_{\text{el}}}{E_{\text{th}}}} \right). \tag{S-83}$$

Apparently, the root is always positive. As consequence, the two eigenvalues are from mutually different number-fields (since $\tilde{\alpha}_1 < 0$ leads to oscillations, whereas $\tilde{\alpha}_2 > 0$ leads to exponentially damped profiles). Since the general solution is the superposition of the two solutions determined by the two eigenvalues, this leads to a superposition of an exponentially damped profile, and an undamped oscillatory profile. Depending upon the amplitudes of these two solutions (*i.e.* the boundary conditions), there exists a plethora of possible screening profiles. However, in all cases, an undamped oscillatory contribution appears, although it may have a very small amplitude. This situation does not occur for positive parameters $\mathcal{V}^0$, where the eigenvalues are always from the same number-field.

Like in the previous case, the phase boundary is minimal for symmetric ions ($\gamma_\pm = 1/2$). Hence, entropy is more dominant when the size-asymmetry between the ion-species is large.

# S-4 Simulations

## S-4.1 Computational Details

Our simulation set up consists of a one-dimensional system composed of the IL-electrolyte, and two ideal planar electrodes separated by the system length $L = 60\,\text{nm}$. The system length is sufficiently large to contain the EDL structures, and the electroneutral regions in the cases where the screening profiles exhibit exponentially damped shape, and damped oscillatory shape. We erect an equidistant spatial grid and implement the system in Matlab, which we solve simultaneously for charge density, and the electric potential. Thus, we do not consider chemical interactions between electrolyte and the electrodes, and chemical reactions are not considered. The corresponding system of equations consists of differential and algebraic equations, and is solved using the fully

implicit Matlab solver ode15s.

We start from the equilibrium state of the system and increase the overpotential from zero up to the terminal value $\Delta\phi$. Thereby, we set the potential of zero charge to zero, $\Phi_{pzc} = 0$. Furthermore, we neglect specific adsorption of ions at the electrode surface.

### S-4.2 Binary Ionic Liquid PyrTFSI

The parameters for the Ionic Liquid $PYR_{1,4}TFSA$ (structure formula $C_{11}H_{20}F_6N_2O_4S_2$) are enlisted in table S-2. The parameters for mass density and conductivity of the ionic liquid have been measured by Iolitec.[S4] The value for the relative dielectric constant is taken from the literature.[S11] The ion-size was estimated (see also Ref. S4). The molar masses were calculated from the structure formulas of the IL-ions (structure formula of $PYR_{1,4}$: $C_9H_{20}N$; structure formula of TFSA: $C_2F_6N_2O_4S_2$)

**Table S-2: Simulation parameters for the neat ionic liquid $Pyr_{1,4}$TFSA.**

| Parameter | Value | Source |
|---|---|---|
| Density $\rho$ / kg m$^{-3}$ | $1.4\times10^3$ | Ref. S4 |
| Electric conductivity $\kappa$ / S m$^{-1}$ | $2.1\times10^{-1}$ | Ref. S4 |
| Dielectric constant $\varepsilon_R$ / - | $1.5\times10^1$ | Ref. S11 |
| Ion size $a/2$ / nm | 0.67 | Ref. S4 |
| Molar mass $M_{PYR_{1,4}}$ / kg mol$^{-1}$ | $142.3\times10^{-3}$ | Calculated |
| Molar mass $M_{TFSA}$ / kg mol$^{-1}$ | $280.1\times10^{-3}$ | Calculated |

## S-5 Relation to Experimental Methods

AFM force curve measurements are often used for the experimental examination of interfacial IL-structures near electrified interfaces.[S12] This type of scanning probe microscope uses sharp tips attached to micro-cantilevers in order to probe forces $F^{AFM}$, appearing between the interface and the liquid sample (IL), as function of electrode distance. The corresponding force-profiles usually depict a damped oscillatory shape. The "wave-length" of the oscillations, *i.e.* the distance between

consecutive peaks of $F^{\mathrm{AFM}}$, is usually attributed to the ion-size.[S13] In addition, the number of peaks provides a means for evaluating the interaction strength. The corresponding EDL-forces appearing in our framework are[S4]

$$F^{\mathrm{EDL}} = \frac{\nu \varrho}{F} \cdot \nabla \Phi. \tag{S-84}$$

Comparing the frequency and number of peaks in the profiles of $F^{\mathrm{AFM}}$ and $F^{\mathrm{EDL}}$ provides a means for qualitative validation of our theory.[S4] However, in contrast to the nano-scaled tip of the cantilever, which penetrates the highly crystalline structure, eq. (S-84) accounts for elastic perturbations thereof. Thus, the absolute scale of magnitude for the amplitudes of $F^{\mathrm{AFM}}$ and $F^{\mathrm{EDL}}$ usually differs.[S4]

# S-6 Simulation Results

In this section, we supplement the simulation results shown in the main text, see section IV C. First, in section S-6.1 we show the phase space as functions of ion-size, ion asymmetry and valency. Next, in section S-6.2 we focus on phase separation in the limit of very large interaction energies. Finally, in section S-6.4, we show that the peak-variance defined in the main text converges. Also, we discuss the peak-number as function of the interaction energy.

## S-6.1 Phase Space of Screening Profiles

In fig. S-1, we supplement the phase diagrams shown in the main text (see fig. 4), and consider the influence of ion-size $a$, ion-asymmetry $\gamma_+$ and valency $z_+$ on the phase boundaries. The left figure shows that the intermediate screening phase of damped oscillations gets suppressed for larger ions. The figure in the middle shows that the two phase boundaries are minimal for symmetric ions $\gamma_\pm = 0.5$ (due to $\gamma_- = 1 - \gamma_+$ it suffices to restrict the discussion to $\gamma_+$). The figure on the right shows the screening phases for two different ion-valencies. Apparently, the intermediate screening phase corresponding to monovalent ion-species ($z_+ = 1$) is smaller than for the case of $z_+ = 2$.

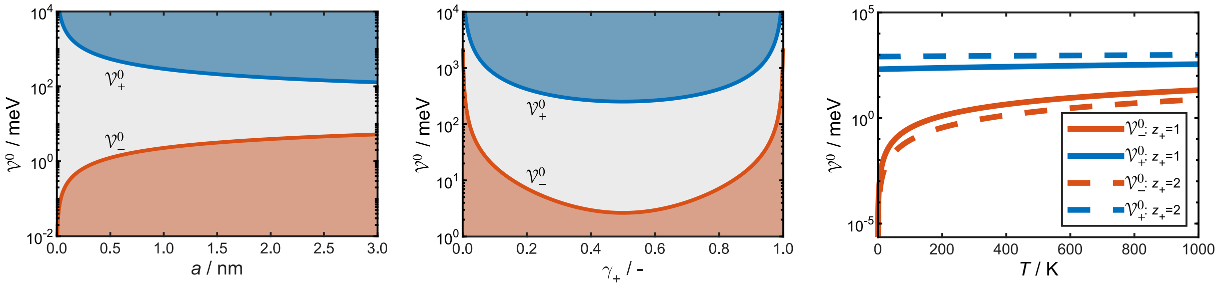


Figure S-1: Phase diagrams for the screening phases as functions ion-size $a$, ion-asymmetry $\gamma_\pm$, and as function of ion-valency $z_+$ (see eq. (45)). In all three figures, the red line indicates the phase boundary $\mathcal{V}^0_-$, whereas the blue line indicates the phase-boundary $\mathcal{V}^0_+$. Left figure: $T = 300\,\mathrm{K}$, $\varepsilon_\mathrm{R} = 15$, and $\gamma = 0.5$. Figure in the middle: $T = 300\,\mathrm{K}$, $\varepsilon_\mathrm{R} = 15$, and $a = 1.3\,\mathrm{nm}$. Right figure: $T = 300\,\mathrm{K}$, $\varepsilon_\mathrm{R} = 15$, $\gamma = 0.5$, and $a = 1.3\,\mathrm{nm}$.

## S-6.2 Crystalline Limit: Ionic Phase-Separation

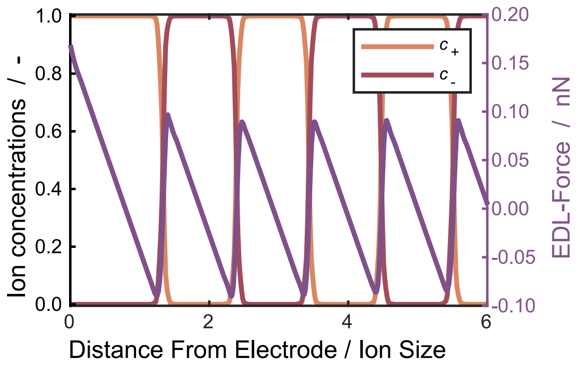


Figure S-2: Numerical results for the ion-concentrations and the double-layer forces over the first six ion-layers at $\mathcal{V}^0 = 500\,\mathrm{meV}$. The left $y$-axis shows the species concentrations $c_\pm$ as obtained from the integral description (eqs. (18) and (19)). The right $y$-axis corresponds to the double-layer forces $F^\mathrm{EDL}$ as obtained from eq. (S-84).

In fig. S-2 we highlight the occurrence of phase separation in the bulk IL-electrolyte for the case $\mathcal{V}^0 \gg E_\mathrm{el}, E_\mathrm{th}$ (here $\mathcal{V}^0 = 500\,\mathrm{meV}$, $\Delta\phi = -100\,\mathrm{mV}$). This figure shows the ion-concentrations (left $y$-axis), and the double-layer forces eq. (S-84) (right $y$-axis) corresponding to the first six ion-layers adjacent to the negatively charged interface. This illustration details the charge-profile shown in fig. 6. Both, the concentration profile, as well as the profile of the double-layer forces exhibit sharply separated ion-layers of box-shaped form. The width of the ion-layers scale exactly with $a$,

*i.e.* the size of the ions.

### S-6.3 Dependence of the Screening Profile on the Interface Potential

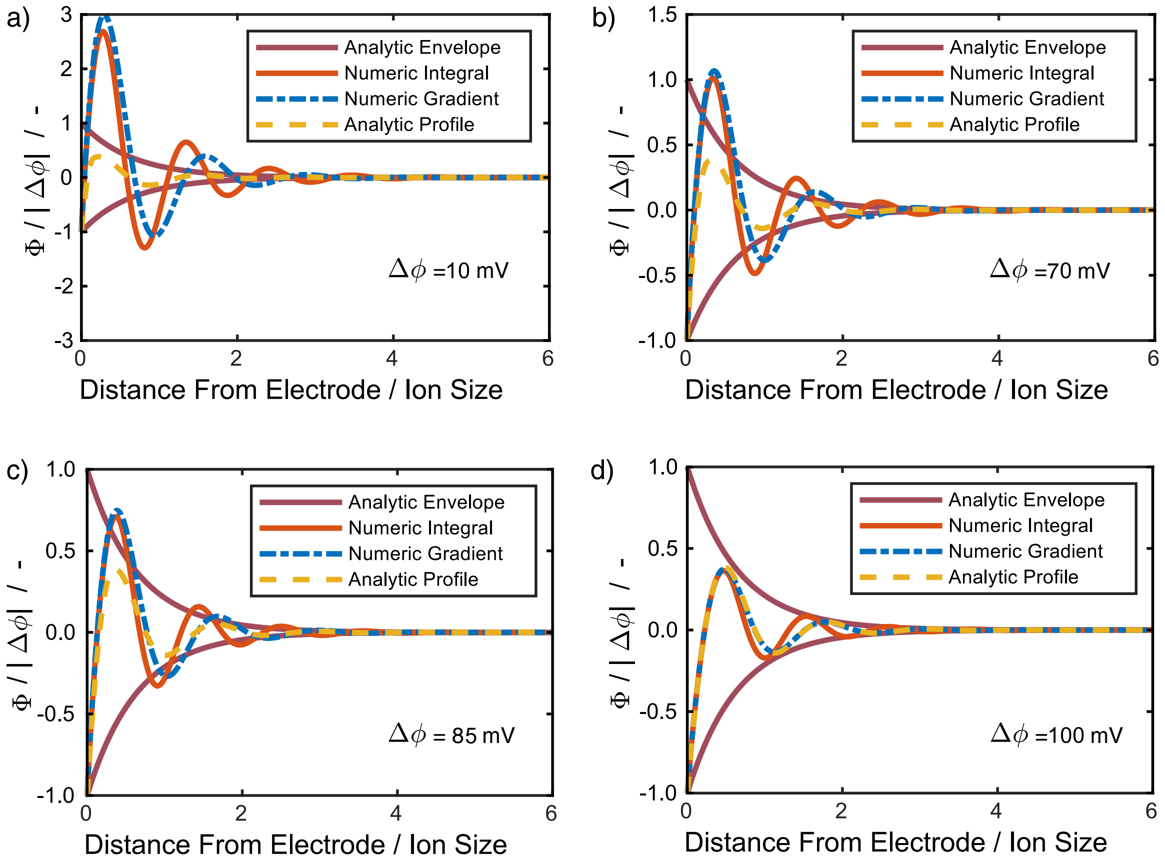


Figure S-3: Numerical results for the electrolyte electric potentials at different values for the interface-overpotential $\Delta\Phi$.

In this section, we discuss the influence of the interface-potential $\Delta\phi$ on the screening profile of the electrolyte electric potential $\Phi$. For this purpose, we compare the numerical results and the analytical prediction for $\Phi$ at constant interaction energy for varying boundary conditions $\Delta\phi$.

Figure S-3 shows the numerical results and the analytical prediction for the electrolyte electric potential $\Phi$ at $\mathcal{V}^0 = 180\,\mathrm{meV}$ for boundary-values $\Delta\phi \in \{10\,\mathrm{meV}, 70\,\mathrm{meV}, 85\,\mathrm{meV}, 100\,\mathrm{meV}\}$. We infer several conclusions from the four figures a)-d).

First, we focus on the comparison of the numerical results stemming from the integral description (see eqs. (18) and (19)) and the gradient description (see eqs. (18) and (23)). By comparison of figures a)-d) we observe that the boundary condition influences the agreement between the two different numerical results only in the region of the first few ion-sizes adjacent to the electrode. Apparently, for larger interface-potentials $\Delta\phi$, the agreement between both profiles increases. Thus, the discrepancy between the two EDL-descriptions near the interface depends upon the boundary condition. In contrast, we observe a good agreement between the numerical results of the gradient expansion and the analytical predictions in the region far away from the electrode in all four cases, *i.e.* independently from the applied electrode-potential $\Delta\phi$.

Next, we focus on the numerical results close to the interface. For $\Delta\phi = 10\,\mathrm{meV}$ the amplitude of the first oscillation-peak "overshoots" the interfacial value significantly for small interface-potentials (roughly by a factor of three, see figure a) in both numerical profiles. With increasing magnitude of $|\Delta\phi|$, this "overscreening" close to the interface decreases, as the amplitude of the first peak decreases relative to the boundary-value. Interestingly, the amplitude of the first oscillation-peak equals almost exactly the boundary value at $\Delta\phi = 70\,\mathrm{meV}$ (see figure b), which is roughly the saturation threshold in the bulk-description (see fig. 2 in the main text). For enhanced potentials $\Delta\phi$, the first amplitude becomes smaller than the boundary-value. The overscreening effect is thus potential-dependent.

Finally, we compare the numerical results with the analytical prediction. By construction, the analytical profile shown in the normalized scaling is independent from the boundary condition. As discussed above, the overscreening of the numerical results in the first oscillation peak decreases with increasing interface-potental. Thus, the agreement between the numerical results and the analytical prediction is potential-dependent only close to the interface.

## S-6.4 Meta Analysis of EDL-Descriptions

In the main text, we introduced the variance of the peak numbers $\sigma(\mathcal{V}^0)$, see eq. (55). Here, we first show that this quantity converges to a limiting value in the case when $\mathcal{V}^0_+ \ll \mathcal{V}^0$. Next, we

discuss the peak-number as function of interaction energy.

Let us consider the limit where the interaction energy $\mathcal{V}_+^0 \ll \mathcal{V}^0$. In this case, the screening profile exhibits undamped oscillations. Furthermore, the amplitude of the peaks are saturated, *i.e.* $\tilde{\varrho}_i = 1$ for all $i$. The corresponding width of the ion layers is determined by the ion-sizes $a$ (see fig. S-2 and eq. (48)). Thus, the saturated peaks are, to a good approximation, located at $x_i = a \cdot i$, and the length of the layered electrolyte $L_{\text{cell}}$ can be approximated via $L_{\text{cell}} \approx \mathrm{N}_{\text{peaks}} \cdot a$. Using Faulhaber's formula,[S14] it is easy show that the variance becomes in this limit

$$\sigma^2 \approx \frac{a^2}{\mathrm{N}_{\text{peaks}}} \cdot \sum_{i=1}^{\mathrm{N}_{\text{peaks}}} i^2 = a^2 \cdot \left( \frac{\mathrm{N}_{\text{peaks}}^2}{3} + \frac{\mathrm{N}_{\text{peaks}}}{2} + \frac{1}{6} \right). \tag{S-85}$$

However, for large values $\mathrm{N}_{\text{peaks}}$ (here, $\mathrm{N}_{\text{peaks}} \approx 90$), the right side of eq. (S-85) converges to $a^2 \cdot \mathrm{N}_{\text{peaks}}^2/3$. Hence, we find that

$$\sigma \to \frac{a \cdot \mathrm{N}_{\text{peaks}}}{\sqrt{3}} \approx \frac{L_{\text{cell}}}{\sqrt{3}}. \tag{S-86}$$

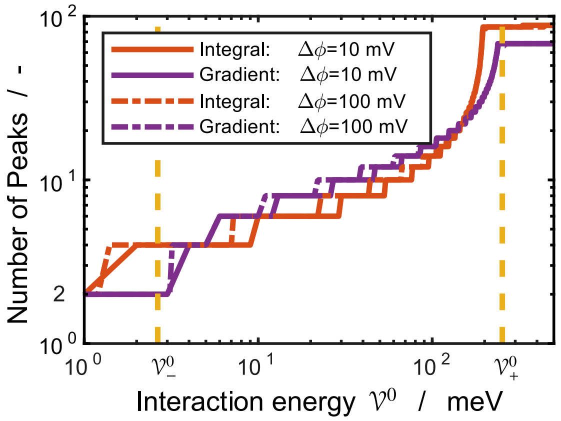


Figure S-4: Meta analysis of the number of peaks occurring in roughly 3000 EDL simulations (see also fig. 9). See eqs. (18) and (19) for the integral description, and eqs. (18) and (23) for the gradient description. The vertical yellow dashed lines show the analytical predictions for the phase-boundaries, see eq. (45).

Figure S-4 shows the number of peaks occurring in the full-cell profiles as function of the

interaction energy $\mathcal{V}^0$ for two different boundary conditions $\Delta\phi$. It relates to the meta-analysis presented in fig. 9, see the main text. The dashed vertical yellow lines are the phase-boundaries $\mathcal{V}^0_\pm$, as predicted by our analytical description (see eq. (45)). The solid and dashed blue lines show the results corresponding to the Gradient description (see eqs. (18) and (23)).

For small interaction energies $\mathcal{V}^0 < \mathcal{V}^0_-$, the peak-number of the gradient description is two. This corresponds to exponentially damped profiles discussed in section III A, *i.e.* charge-saturation at the two oppositely charged interfaces. For energies $\mathcal{V}^0 = \mathcal{V}^0_-$, the number of peaks starts increasing step-wise with increasing $\mathcal{V}^0$. Apparently, for energies close to $\mathcal{V}^0_+$ the increase becomes exponential and converges to a plateau of maximal peak-number, exactly at $\mathcal{V}^0 = \mathcal{V}^0_+$. This corresponds to the situation where the complete bulk electrolyte has undergone a phase separation into ionic layers. Apparently, the number of maximal peaks (roughly 80) is smaller than the length of the cell divided by the ion-size (roughly 90). This can be attributed to the fact that the gradient approximation slightly underestimates the interaction strength.

The solid and dashed red lines show the results corresponding to the integral description (see eqs. (18) and (19)). Apparently, the number of peaks increases above two (no oscillations) for energies $\mathcal{V}^0 < \mathcal{V}^0_-$, *i.e.* the profiles start oscillating slightly below the analytically predicted phase boundary at $\mathcal{V}^0_- = 3\,\mathrm{meV}$. Next, the number of oscillations shows step-wise increase with $\mathcal{V}^0$, followed by an exponential increase with $\mathcal{V}^0$ starting above $100\,\mathrm{meV}$. However, at roughly $\mathcal{V}^0 = 200\,\mathrm{meV}$, the profile converges into a constant plateau of maximal peak-number (roughly 90 peaks). Thus, the bulk electrolyte undergoes phase-separation into ionic layers at interaction energies slightly smaller than the analytical prediction. Thus, both phase-boundaries in the integral description are shifted to smaller values of $\mathcal{V}^0$. $\mathcal{V}^0_i < \mathcal{V}^0_-$. This is in accordance with the variance $\sigma$, see fig. 9. Finally, we note that the step-wise increase for of the peak-numbers (at moderate interaction energies) in both descriptions is not an artifact of a discrete set of simulations (the increment in the simulations is roughly $\Delta\mathcal{V}^0 = 0.1\,\mathrm{meV}$).

# References


(S1) Schammer, M.; Horstmann, B.; Latz, A. Theory of Transport in Highly Concentrated Electrolytes. *Journal of the Electrochemical Society* **2021**, *168*, 026511.

(S2) Henjes, K.; Liu, M. Hydrodynamics of Polarizable Liquids. *Annals of Physics* **1993**, *223*, 243–276.

(S3) Kovetz, A. *Electromagnetic theory*; Oxford University Press Oxford, 2000; Vol. 975.

(S4) Hoffmann, V.; Pulletikurthi, G.; Carstens, T.; Lahiri, A.; Borodin, A.; Schammer, M.; Horstmann, B.; Latz, A.; Endres, F. Influence of a silver salt on the nanostructure of a Au(111)/ionic liquid interface: an atomic force microscopy study and theoretical concepts. *Phys. Chem. Chem. Phys.* **2018**, *20*, 4760–4771.

(S5) Gavish, N.; Yochelis, A. Theory of Phase Separation and Polarization for Pure Ionic Liquids. *The Journal of Physical Chemistry Letters* **2016**, *7*, 1121–1126.

(S6) Van Dijk, M.; Wakker, A. *Concepts in polymer thermodynamics*; CRC Press, 1998; Vol. 2.

(S7) Bothe, D.; Dreyer, W.; Druet, P.-E. Multicomponent incompressible fluids – An asymptotic study. 2021.

(S8) Bazant, M. Z.; Storey, B. D.; Kornyshev, A. A. Double Layer in Ionic Liquids: Overscreening versus Crowding. *Phys. Rev. Lett.* **2011**, *106*, 046102.

(S9) Parr, R. G. *Horizons of quantum chemistry*; Springer, 1980; pp 5–15.

(S10) Schmickler, W.; Santos, E. *Interfacial electrochemistry*; Springer Science & Business Media, 2010.

(S11) Huang, M.-M.; Jiang, Y.; Sasisanker, P.; Driver, G. W.; Weingärtner, H. Static Relative Dielectric Permittivities of Ionic Liquids. *Journal of Chemical & Engineering Data* **2011**, *56*, 1494–1499.

(S12) Rodenbücher, C.; Wippermann, K.; Korte, C. Atomic Force Spectroscopy on Ionic Liquids. *Applied Sciences* **2019**, *9*.

(S13) Li, H.; Endres, F.; Atkin, R. Effect of alkyl chain length and anion species on the interfacial nanostructure of ionic liquids at the Au(111)âĂŞionic liquid interface as a function of potential. *Phys. Chem. Chem. Phys.* **2013**, *15*, 14624–14633.

(S14) Knuth, D. E. Johann Faulhaber and sums of powers. *Mathematics of Computation* **1993**, *61*, 277–294.
